# Supplementary material for: On the Convergence of Adam-Type Algorithm for Bilevel Optimization under Unbounded Smoothness
Source: arXiv:2503.03908 source file (2025-03-05)
Supplement: Supplementary file 1 [file proof_sketch_vr.tex]

For VR-AdamBO, we provide a more detailed proof sketch here due to space constraints in the main text. In particular, we present two main challenges and outline the proof roadmap to address them.

\paragraph{\textbf{Challenge 1: VR-AdamBO vs. VRAdam \citep{li2023convergence}}.}

The analysis of VRAdam in the single-level generalized smooth optimization setting~\citep{li2023convergence} is not directly applicable to bilevel problems. This is because the hypergradient estimator in bilevel optimization may have a non-negligible bias due to inaccurate estimation of the lower-level variable, whereas the single-level analysis in~\citep{li2023convergence} does not need to account for this issue. To control the lower-level estimation error, we leverage the lower-level acceleration technique~\citep{gong2024accelerated} with periodic updates and averaging. While we largely adopt the framework of VRAdam for the upper-level analysis, the main distinction lies in our incorporation of the hypergradient bias---arising from inaccurate estimates of the optimal lower-level variable at each iteration---into the upper-level analysis. This is detailed in Lemmas E.5 to E.8 of our paper, which correspond to Lemmas D.4, D.6, D.7, and D.8 in \citep{li2023convergence}, respectively.

\paragraph{\textbf{Challenge 2: VR-AdamBO vs. AccBO \citep{gong2024accelerated}}.}

Although both VR-AdamBO and AccBO \cite{gong2024accelerated} use the same lower-level update (periodic SNAG with averaging) and adopt the same variance reduction technique STORM \citep{cutkosky2019momentum} for the first-order momentum update, the key difference between these two algorithms lies in the upper-level update: AccBO uses normalized SGD with momentum, while VR-AdamBO employs VRAdam. This distinction leads to significantly different theoretical analyses for VR-AdamBO and AccBO. In particular, for VR-AdamBO, we introduce a novel stopping time approach in the context of bilevel optimization (see equation (7) in Section 5.3), building on the VR-Adam analysis \cite{li2023convergence}. Base on the definition of stopping time $\tau$, we develop a new induction argument (i.e., Lemmas E.10 to E.12) to show that under $t<\tau$ and some good event $\gE_y$ (see Lemma E.10 for definition), both $\|\hy_t-y_t^*\|$ and $\|m_t\|$ are bounded. We then show the averaged lower-level error is small (see Lemma E.4) under the parameter choices in Theorem 5.1, which shares an similar spirit as Lemma 4.6 for AdamBO. Combining the aforementioned lemmas with the upper-level analysis mentioned above in Challenge 1 (i.e., Lemmas E.5 to E.8), we can obtain the improved $\widetilde{O}(\epsilon^{-3})$ complexity result.
