# Supplementary material for: On the Convergence of Adam-Type Algorithm for Bilevel Optimization under Unbounded Smoothness
Source: arXiv:2503.03908 source file (2025-03-05)
Supplement: Supplementary file 2 [file proof_vr_adambo.tex]

In this section, we provide convergence analysis for VR-AdamBO (\cref{alg:vradambo}). Before presenting the lemmas and the main theorem, we first define (or restate) a few key concepts and useful notations.

\subsection{Technical Definitions and Useful Notations}
\label{sec:vradambo-notations}

\paragraph{Filtration.}
Let $\sigma(\cdot)$ be the $\sigma$-algebra generated by the random variables within the argument.
Define $\gF_{\init}$ as the filtration for updating $y_1$ (i.e., the filtration of warm-start phase):
\begin{equation*}
    \gF_{\init} = \sigma(\Tilde{\pi}_0,\dots,\Tilde{\pi}_{T_0-1}),
\end{equation*}
% where $\sigma(\cdot)$ denotes the $\sigma$-algebra generated by the random variables within the argument.
For any $t \geq 2$, define $\gF_t^x$ as the filtration of the randomness used in updating $x_t$ before the $t$-th iteration:
\begin{equation*}
    % \gF_t^{\init} = \sigma(\pi_1,\dots,\pi_{t-1}),
    % \quad
    \gF_t^x = \sigma(\gS_1,\Bar{\xi}_2,\dots,\Bar{\xi}_{t-1}),
    \quad
    % \gF_t^y = \sigma(\zeta_1,\dots,\zeta_{t-1}),
\end{equation*}
also define $\gF_t^y$ as the filtration of the randomness used in updating $y_t$ when $t$ is a multiple of $I$:
\begin{equation*}
    \gF_t^y = \sigma(\pi_t^0,\dots,\pi_t^{N-1}).
\end{equation*}
Additionally, let $\gF_t$ denote the filtration of all randomness before the $t$-th iteration:
\begin{equation*}
    \gF_t = \sigma(\gF_{\init} \cup \gF_t^x \cup (\cup_{k<t}\gF_k^y)).
\end{equation*}

\paragraph{Expectation.}
We use $\E_t[\cdot]$ to denote the conditional expectation $\E[\cdot \mid \gF_t]$.

\paragraph{Other Definitions.}
We define the deviation of the momentum from the conditional expectation of the hypergradient estimator as
\begin{equation}
    \epsilon_t \coloneqq m_t - \E_t[\hatphi(x_t,y_t;\Bar{\xi}_t)].
\end{equation}
Also, let $h_t$ be the learning rate vector and $H_t$ be the learning rate matrix:
\begin{equation*}
    h_t \coloneqq \frac{\eta}{\sqrt{\hv_t}+\lambda}
    \quad\quad\text{and}\quad\quad
    H_t \coloneqq \diag(h_t).
\end{equation*}
Then the update rule for upper-level variable $x_t$ (line 18 of \cref{alg:vradambo}) can be written as
\begin{equation*}
    x_{t+1} = x_t - h_t\odot\hm_t = x_t - H_t\hm_t.
\end{equation*}

\paragraph{Stopping Time.}
Given a large enough constant $G$ as defined in \cref{thm:vr-main-appendix}, denote $L$ and $\psi$ as
\begin{equation*}
    L = L_0 + L_1G
    \quad\quad\text{and}\quad\quad
    \psi = \frac{C_LG^2}{2L},
\end{equation*}
where constants $L_0,L_1$ and $C_L$ are defined in \eqref{eq:L0-L1} and \eqref{eq:Cu-def}. Now we formally define the stopping time $\tau$ as
\begin{equation}
    \tau \coloneqq \min\{t \mid \Phi(x_t)-\Phi^* > \psi\} \wedge \min\{t \mid \|\epsilon_t\|>G\} \wedge (T+1).
\end{equation}
Based on \cref{lm:reverse-PL}, we know if $t<\tau$, we have $\Phi(x_t)-\Phi^*\leq \psi$, $\|\epsilon_t\|\leq G$ and $\|\gdphi(x_t)\|\leq G$.

\paragraph{Constants.}
We define the following constants, which will be useful for analysis.
\begin{equation*}
    L = L_0 + L_1G,
    \quad
    \Delta_1 = \Phi(x_1) - \Phi^*,
    \quad
    C_{m} = 2G + \frac{l_{g,1}l_{f,0}}{\mu} + Lr,
    \quad
    C_{\eta} = \frac{512e\Delta_1\sigma_{\phi}LG^2}{c_1\lambda^2\delta^{3/2}\epsilon^3},
\end{equation*}
\begin{equation*}
    \varrho_{\max} = \max_{k\leq \lfloor T/I \rfloor}\|y_{kI+1}-y_{kI}^*\|,
    \quad
    \hrho_{\max} = \max_{t\leq T}\|\hy_t-y_t^*\|,
\end{equation*}
\begin{equation*}
    \hrho 
    = \left(\|\hy_1-y_0^*\| + \eta + \frac{\eta l_{g,1}}{\lambda\mu}\left(\frac{1-\nu}{\nu} + I\right)\left(2G + \frac{l_{g,1}l_{f,0}}{\mu}\right)\right) \Big/ \left(1-\frac{\eta l_{g,1}L}{\lambda\mu}\left(\frac{1-\nu}{\nu} + I\right)\right).
\end{equation*}
Besides, constants $L_0,L_1$ are defined in \eqref{eq:L0-L1}, $r$ is defined in \eqref{eq:r-def}, and $\sigma_{\phi}$ is defined in \cref{sec:adambo-notations}, respectively.

%%%%%%%%%%%%%%%%%%%%%%%%%%%%%%%%%%%%%%%%%%%%%%%%%%%%%%%%%%%%%%%%%%%%%%%%%%%%%%%%%%%%%%%%%%%%%%%

\subsection{Auxiliary Lemmas}
First note that when $t<\tau$, some of the quantities in \cref{alg:vradambo,sec:vradambo-notations} are bounded almost surely. In particular, we have the following lemma.

\begin{lemma} \label{lm:vr-gradient-bound}
If $t<\tau$, we have
\begin{equation*}
    \|\gdphi(x_t)\| \leq G,
    \quad
    \|\epsilon_t\| \leq G,
    \quad
    h_t \preceq \frac{\eta}{\lambda};
\end{equation*}
further, if $\|\hy_t-y_t^*\|\leq r$, then we have
\begin{equation*}
    \|m_t\|
    \leq \|\gdphi(x_t)\| + \|\epsilon_t\| + L\|\hy_t-y_t^*\| + \frac{l_{g,1}l_{f,0}}{\mu}\left(1-\frac{\mu}{l_{g,1}}\right)^Q 
    % \leq \|\gdphi(x_t)\| + \|\epsilon_t\| + L\hrho_{\max} + \frac{l_{g,1}l_{f,0}}{\mu}\left(1-\frac{\mu}{l_{g,1}}\right)^Q,
    % \quad\text{where}\quad
    % \hrho_{\max} \coloneqq \max_{t\leq T}\|\hy_t-y_t^*\|.
\end{equation*}
\end{lemma}

\begin{proof}[Proof of \cref{lm:vr-gradient-bound}]
For the first three results, the proof is the same as \cref{lm:gradient-bound}. For the third one, if $t<\tau$ and $\|\hy_t-y_t^*\|\leq r$, we have
\begin{equation*}
    \begin{aligned}
        \|m_t\|
        &\leq \|m_t-\E_t[\hatphi(x_t,\hy_t;\Bar{\xi}_t)]\| + \|\E_t[\hatphi(x_t,\hy_t;\Bar{\xi}_t)] - \E_t[\hatphi(x_t,y_t^*;\Bar{\xi}_t)]\| \\
        &\quad+ \|\E_t[\hatphi(x_t,y_t^*;\Bar{\xi}_t)] - \gdphi(x_t)\| + \|\gdphi(x_t)\| \\
        &\leq \|\gdphi(x_t)\| + \|\epsilon_t\| + (L_0+L_1\|\gdphi(x_t)\|)\|\hy_t-y_t^*\| + \frac{l_{g,1}l_{f,0}}{\mu}\left(1-\frac{\mu}{l_{g,1}}\right)^Q \\
        &\leq \|\gdphi(x_t)\| + \|\epsilon_t\| + L\|\hy_t-y_t^*\| + \frac{l_{g,1}l_{f,0}}{\mu}\left(1-\frac{\mu}{l_{g,1}}\right)^Q,
        % \leq C_m,
    \end{aligned}
\end{equation*}
where the second inequality uses the definition of $\epsilon_t$, \cref{lm:hyper-stoc-bias,lm:neumann-error}, the third inequality is due to $\|\gdphi(x_t)\|\leq G$ if $t<\tau$, and the definition of $\hrho_{\max}$.
% and the last inequality again uses the definitions of $\nu$ and $C_m$ in \eqref{eq:vr-mt-bound}.
\end{proof}

%%%%%%%%%%%%%%%%%%%%%%%%%%%%%%%%%%%%%%%%%%%%%%%%%%%%%%%%%%%%%%%%%%%%%%%%%%%%%%%%%%%%%%%%%%%%%%%
Next, we provide an upper bound for $\|y_t-y_t^*\|$ using the structure of periodic updates.

\begin{lemma} \label{lm:vr-yt-max-error}
For any $t\geq 1$, we have
\begin{equation*}
    \begin{aligned}
        \|y_t-y_t^*\| 
        \leq \varrho_{\max} + \frac{\eta l_{g,1}}{\lambda\mu}\sum_{i=k_tI}^{t-1}\|m_i\|,
        \quad\text{where}\quad
        \varrho_{\max} \coloneqq \max_{k\leq \lfloor T/I \rfloor}\|y_{kI+1}-y_{kI}^*\|,
    \end{aligned}
\end{equation*}
where $k_t=\lfloor t/I \rfloor$ and we define $m_0=0$ for completeness.
\end{lemma}

\begin{proof}[Proof of \cref{lm:vr-yt-max-error}]
For any $k_tI+1\leq t\leq (k_t+1)I$, we have
\begin{equation*}
    \begin{aligned}
        \|y_t-y_t^*\| 
        &\leq \|y_{kI+1}-y_{kI}^*\| + \sum_{i=k_tI}^{t-1}\|y_i^*-y_{i+1}^*\| 
        \leq \varrho_{\max} + \sum_{i=k_tI}^{t-1}\|y_i^*-y_{i+1}^*\| \\
        &\leq \varrho_{\max} + \frac{l_{g,1}}{\mu}\sum_{i=k_tI}^{t-1}\|x_{i+1}-x_i\| 
        \leq \varrho_{\max} + \frac{\eta l_{g,1}}{\lambda\mu}\sum_{i=k_tI}^{t-1}\|m_i\|,
    \end{aligned}
\end{equation*}
where the second inequality uses the definition of $\varrho_{\max}$, the third inequality is due to \eqref{lm:lip-y}, and the last inequality uses the update rule in \cref{alg:vradambo} and \cref{lm:vr-gradient-bound}.
\end{proof}

%%%%%%%%%%%%%%%%%%%%%%%%%%%%%%%%%%%%%%%%%%%%%%%%%%%%%%%%%%%%%%%%%%%%%%%%%%%%%%%%%%%%%%%%%%%%%%%
The following lemma provides bound for the lower-level estimation error.

\begin{lemma} \label{lm:average}
Consider the averaging step (line 15) of \cref{alg:vradambo}, for any $t\geq 1$ we have
\begin{equation*}
    \begin{aligned}
        \|\hy_t-y_t^*\|
        \leq (1-\nu)^{t-1}\|\hy_1-y_0^*\| + \frac{(1-\nu)\eta l_{g,1}}{\lambda\mu}\sum_{i=1}^{t}(1-\nu)^{t-i}\|m_{i-1}\| + \nu\sum_{i=1}^{t}(1-\nu)^{t-i}\|y_i-y_i^*\|.
    \end{aligned}
\end{equation*}
\end{lemma}

\begin{proof}[Proof of \cref{lm:average}]
Define $\hy_0=y_0$ for simplicity. By the update rule of $\hy_t$, we have
\begin{equation*}
    \begin{aligned}
        \|\hy_t-y_t^*\|
        &= \|(1-\nu)(\hy_{t-1}-y_t^*) + \nu(y_t-y_t^*)\| \\
        &= \|(1-\nu)(\hy_{t-1}-y_{t-1}^*) + (1-\nu)(y_{t-1}^*-y_t^*) + \nu(y_t-y_t^*)\| \\
        &\leq (1-\nu)\|\hy_{t-1}-y_{t-1}^*\| + (1-\nu)\|y_{t-1}^*-y_t^*\| + \nu\|y_t-y_t^*\|.
    \end{aligned}
\end{equation*}
We apply the above inequality recursively to obtain
\begin{equation*}
    \begin{aligned}
        \|\hy_t-y_t^*\| 
        &\leq (1-\nu)^{t-1}\|\hy_1-y_1^*\| + (1-\nu)\sum_{i=2}^{t}(1-\nu)^{t-i}\|y_{i-1}^*-y_i^*\| + \nu\sum_{i=2}^{t}(1-\nu)^{t-i}\|y_i-y_i^*\| \\
        &\leq (1-\nu)^{t-1}\|\hy_1-y_0^*\| + \frac{(1-\nu)\eta l_{g,1}}{\lambda\mu}\sum_{i=1}^{t}(1-\nu)^{t-i}\|m_{i-1}\| + \nu\sum_{i=1}^{t}(1-\nu)^{t-i}\|y_i-y_i^*\|,
    \end{aligned}
\end{equation*}
where the last inequality uses $x_1=x_0$ and \cref{lm:lip-y}.
\end{proof}

%%%%%%%%%%%%%%%%%%%%%%%%%%%%%%%%%%%%%%%%%%%%%%%%%%%%%%%%%%%%%%%%%%%%%%%%%%%%%%%%%%%%%%%%%%%%%%%
The following lemma characterizes the averaged lower-level estimation error.

\begin{lemma} \label{lm:sum-hy-and-y}
Under the parameter choices in \cref{thm:vr-main-appendix}, if $\|\hy_t-y_t^*\|\leq r$ holds for all $t$, then we have
\begin{equation*}
    \begin{aligned}
        \sum_{t=1}^{\tau}\|\hy_t-y_t^*\|^2
        &\leq \frac{6}{\nu}\|\hy_1-y_0^*\|^2 + 12\varrho_{\max}^2T \\
        &\quad+ \frac{72l_{g,1}^2}{\lambda^2\mu^2}\left(\frac{\eta^2}{\nu^2} + \eta^2I^2\right)\sum_{t=1}^{\tau-1}\left(\|\gdphi(x_t)\|^2 + \|\epsilon_t\|^2 + \frac{l_{g,1}^2l_{f,0}^2}{\mu^2}\left(1-\frac{\mu}{l_{g,1}}\right)^{2Q}\right)
    \end{aligned}
\end{equation*}
and
\begin{equation*}
    \begin{aligned}
        \sum_{t=1}^{\tau}\|y_t-y_t^*\|^2
        &\leq \frac{48\eta^2l_{g,1}^2I^2L^2}{\nu\lambda^2\mu^2}\|\hy_1-y_0^*\|^2 + \left(2 + \frac{96\eta^2l_{g,1}^2I^2L^2}{\lambda^2\mu^2}\right)\varrho_{\max}^2T \\
        &\quad+ \frac{8\eta^2l_{g,1}^2I^2}{\lambda^2\mu^2}\left(1 + \frac{72l_{g,1}^2L^2}{\lambda^2\mu^2}\left(\frac{\eta^2}{\nu^2} + \eta^2I^2\right)\right)\sum_{t=1}^{\tau-1}\left(\|\gdphi(x_t)\|^2 + \|\epsilon_t\|^2\right) \\
        &\quad+ \frac{8\eta^2l_{g,1}^2I^2}{\lambda^2\mu^2}\left(1 + \frac{72l_{g,1}^2L^2}{\lambda^2\mu^2}\left(\frac{\eta^2}{\nu^2} + \eta^2I^2\right)\right)\frac{l_{g,1}^2l_{f,0}^2}{\mu^2}\left(1-\frac{\mu}{l_{g,1}}\right)^{2Q}.
    \end{aligned}
\end{equation*}
\end{lemma}

\begin{proof}[Proof of \cref{lm:sum-hy-and-y}]
If $t\leq \tau$, by \cref{lm:vr-yt-max-error} we have
\begin{equation*}
    \begin{aligned}
        \|y_t-y_t^*\| 
        \leq \varrho_{\max} + \frac{\eta l_{g,1}}{\lambda\mu}\sum_{i=k_tI}^{t-1}\|m_i\|.
        % \leq \varrho + \frac{\eta l_{g,1}}{\lambda\mu}\sum_{i=kI}^{\min\{(k+1)I-1,\nu-1\}}\|m_i\|.
    \end{aligned}
\end{equation*}
Then we have
\begin{equation} \label{eq:vr-yt-and-mi}
    \begin{aligned}
        \|y_t-y_t^*\|^2
        &\leq \left(\varrho_{\max} + \frac{\eta l_{g,1}}{\lambda\mu}\sum_{i=k_tI}^{t-1}\|m_i\|\right)^2 
        \leq 2\varrho_{\max}^2 + \frac{2\eta^2l_{g,1}^2}{\lambda^2\mu^2}\left(\sum_{i=k_tI}^{t-1}\|m_i\|\right)^2 \\
        &\leq 2\varrho_{\max}^2 + \frac{2\eta^2l_{g,1}^2I}{\lambda^2\mu^2}\sum_{i=k_tI}^{t-1}\|m_i\|^2.
    \end{aligned}
\end{equation}

Taking summation on both sides of \eqref{eq:vr-yt-and-mi} over $t$ from 1 to $\nu$, we have
\begin{equation} \label{eq:vr-yt-and-mi-sum}
    \begin{aligned}
        \sum_{t=1}^{\tau}\|y_t-y_t^*\|^2
        &= \sum_{k=0}^{\lfloor \nu/I \rfloor-1}\sum_{t=kI}^{\min\{(k+1)I, \nu\}}\|y_t-y_t^*\|^2 \\
        &\leq \sum_{k=0}^{\lfloor \nu/I \rfloor-1}\sum_{t=kI}^{\min\{(k+1)I, \nu\}}\left(2\varrho_{\max}^2 + \frac{2\eta^2l_{g,1}^2I}{\lambda^2\mu^2}\sum_{i=k_tI}^{t-1}\|m_i\|^2\right) \\
        &\leq 2\varrho_{\max}^2(\nu-1) + \frac{2\eta^2l_{g,1}^2I^2}{\lambda^2\mu^2}\sum_{k=0}^{\lfloor \nu/I \rfloor-1}\sum_{t=kI}^{\min\{(k+1)I, \nu\}}\|m_t\|^2 \\
        &\leq 2\varrho_{\max}^2T + \frac{2\eta^2l_{g,1}^2I^2}{\lambda^2\mu^2}\sum_{t=1}^{\tau-1}\|m_t\|^2,
    \end{aligned}
\end{equation}
where the last inequality uses the definition of $\nu$ and $m_0=0$.

By \cref{lm:average}, we have
\begin{equation*}
    \begin{aligned}
        \sum_{t=1}^{\tau}\|\hy_t-y_t^*\|^2
        &\leq 3\sum_{t=1}^{\tau}(1-\nu)^{2(t-1)}\|\hy_1-y_0^*\|^2 + 3\sum_{t=1}^{\tau}\left(\frac{(1-\nu)\eta l_{g,1}}{\nu\lambda\mu}\nu\sum_{i=1}^{t}(1-\nu)^{t-i}\|m_{i-1}\|\right)^2 \\
        &\quad+ 3\sum_{t=1}^{\tau}\left(\nu\sum_{i=1}^{t}(1-\nu)^{t-i}\|y_i-y_i^*\|\right)^2 \\
        &\leq \frac{3}{\nu}\|\hy_1-y_0^*\|^2 + \frac{3(1-\nu)^2\eta^2 l_{g,1}^2}{\nu^2\lambda^2\mu^2}\sum_{t=1}^{\tau}\nu\sum_{i=1}^{t}(1-\nu)^{t-i}\|m_{i-1}\|^2 \\
        &\quad+ 3\sum_{t=1}^{\tau}\nu\sum_{i=1}^{t}(1-\nu)^{t-i}\|y_i-y_i^*\|^2 \\
        &\leq \frac{3}{\nu}\|\hy_1-y_0^*\|^2 + \frac{3(1-\nu)^2\eta^2 l_{g,1}^2}{\nu^2\lambda^2\mu^2}\sum_{t=1}^{\tau-1}\|m_t\|^2 + 3\sum_{t=1}^{\tau}\|y_t-y_t^*\|^2 \\
        &\leq \frac{3}{\nu}\|\hy_1-y_0^*\|^2 + \frac{3(1-\nu)^2\eta^2 l_{g,1}^2}{\nu^2\lambda^2\mu^2}\sum_{t=1}^{\tau-1}\|m_t\|^2 + 3\left(2\varrho_{\max}^2T + \frac{2\eta^2l_{g,1}^2I^2}{\lambda^2\mu^2}\sum_{t=1}^{\tau-1}\|m_t\|^2\right) \\
        &\leq \frac{3}{\nu}\|\hy_1-y_0^*\|^2 + 6\varrho_{\max}^2T + \frac{9l_{g,1}^2}{\lambda^2\mu^2}\left(\frac{\eta^2}{\nu^2} + \eta^2I^2\right)\sum_{t=1}^{\tau-1}\|m_t\|^2,
    \end{aligned}
\end{equation*}
where the first inequality uses Young's inequality; the second inequality is due to Jensen's inequality; the third inequality uses the sum of geometric series; the fourth inequality is due to \eqref{eq:vr-yt-and-mi-sum}.
By \cref{lm:vr-gradient-bound}, we know that
\begin{equation*}
    \begin{aligned}
        \|m_t\|
        \leq \|\gdphi(x_t)\| + \|\epsilon_t\| + L\|\hy_t-y_t^*\| + \frac{l_{g,1}l_{f,0}}{\mu}\left(1-\frac{\mu}{l_{g,1}}\right)^Q.
    \end{aligned}
\end{equation*}
Then we obtain
\begin{equation*}
    \begin{aligned}
        \sum_{t=1}^{\tau}\|\hy_t-y_t^*\|^2
        &\leq \frac{3}{\nu}\|\hy_1-y_0^*\|^2 + 6\varrho_{\max}^2T \\
        &\quad+ \frac{9l_{g,1}^2}{\lambda^2\mu^2}\left(\frac{\eta^2}{\nu^2} + \eta^2I^2\right)\sum_{t=1}^{\tau-1}\left(\|\gdphi(x_t)\| + \|\epsilon_t\| + L\|\hy_t-y_t^*\| + \frac{l_{g,1}l_{f,0}}{\mu}\left(1-\frac{\mu}{l_{g,1}}\right)^Q\right)^2 \\
        &\leq \frac{3}{\nu}\|\hy_1-y_0^*\|^2 + 6\varrho_{\max}^2T \\
        &\quad+ \frac{36l_{g,1}^2}{\lambda^2\mu^2}\left(\frac{\eta^2}{\nu^2} + \eta^2I^2\right)\sum_{t=1}^{\tau-1}\left(\|\gdphi(x_t)\|^2 + \|\epsilon_t\|^2 + L^2\|\hy_t-y_t^*\|^2 + \frac{l_{g,1}^2l_{f,0}^2}{\mu^2}\left(1-\frac{\mu}{l_{g,1}}\right)^{2Q}\right).
    \end{aligned}
\end{equation*}
Under the parameter choices in \cref{thm:vr-main-appendix}, by \cref{sec:vr-para-verify} we have
\begin{equation*}
    \begin{aligned}
        \frac{36l_{g,1}^2}{\lambda^2\mu^2}\left(\frac{\eta^2}{\nu^2} + \eta^2I^2\right)L^2 \leq \frac{1}{2}.
    \end{aligned}
\end{equation*}
Rearranging the above inequality yields
\begin{equation} \label{eq:vr-haty-sum}
    \begin{aligned}
        \sum_{t=1}^{\tau}\|\hy_t-y_t^*\|^2
        &\leq \frac{6}{\nu}\|\hy_1-y_0^*\|^2 + 12\varrho_{\max}^2T \\
        &\quad+ \frac{72l_{g,1}^2}{\lambda^2\mu^2}\left(\frac{\eta^2}{\nu^2} + \eta^2I^2\right)\sum_{t=1}^{\tau-1}\left(\|\gdphi(x_t)\|^2 + \|\epsilon_t\|^2 + \frac{l_{g,1}^2l_{f,0}^2}{\mu^2}\left(1-\frac{\mu}{l_{g,1}}\right)^{2Q}\right).
    \end{aligned}
\end{equation}
Finally, using the previous results we conclude that
\begin{equation*}
    \begin{aligned}
        \sum_{t=1}^{\tau}\|y_t-y_t^*\|^2
        &\leq 2\varrho_{\max}^2T + \frac{2\eta^2l_{g,1}^2I^2}{\lambda^2\mu^2}\sum_{t=1}^{\tau-1}\|m_t\|^2 \\
        &\leq 2\varrho_{\max}^2T + \frac{2\eta^2l_{g,1}^2I^2}{\lambda^2\mu^2}\sum_{t=1}^{\tau-1}\left(\|\gdphi(x_t)\| + \|\epsilon_t\| + L\|\hy_t-y_t^*\| + \frac{l_{g,1}l_{f,0}}{\mu}\left(1-\frac{\mu}{l_{g,1}}\right)^Q\right)^2 \\
        &\leq 2\varrho_{\max}^2T + \frac{8\eta^2l_{g,1}^2I^2}{\lambda^2\mu^2}\sum_{t=1}^{\tau-1}\left(\|\gdphi(x_t)\|^2 + \|\epsilon_t\|^2 + L^2\|\hy_t-y_t^*\|^2 + \frac{l_{g,1}^2l_{f,0}^2}{\mu^2}\left(1-\frac{\mu}{l_{g,1}}\right)^{2Q}\right) \\
        &\leq 2\varrho_{\max}^2T + \frac{8\eta^2l_{g,1}^2I^2}{\lambda^2\mu^2}\sum_{t=1}^{\tau-1}\left(\|\gdphi(x_t)\|^2 + \|\epsilon_t\|^2 + \frac{l_{g,1}^2l_{f,0}^2}{\mu^2}\left(1-\frac{\mu}{l_{g,1}}\right)^{2Q}\right) \\
        &\quad+ \frac{8\eta^2l_{g,1}^2I^2L^2}{\lambda^2\mu^2}\left(\frac{6}{\nu}\|\hy_1-y_0^*\|^2 + 12\varrho_{\max}^2T \right. \\
        &\left.\quad+ \frac{72l_{g,1}^2}{\lambda^2\mu^2}\left(\frac{\eta^2}{\nu^2} + \eta^2I^2\right)\sum_{t=1}^{\tau-1}\left(\|\gdphi(x_t)\|^2 + \|\epsilon_t\|^2 + \frac{l_{g,1}^2l_{f,0}^2}{\mu^2}\left(1-\frac{\mu}{l_{g,1}}\right)^{2Q}\right)\right) \\
        &= \frac{48\eta^2l_{g,1}^2I^2L^2}{\nu\lambda^2\mu^2}\|\hy_1-y_0^*\|^2 + \left(2 + \frac{96\eta^2l_{g,1}^2I^2L^2}{\lambda^2\mu^2}\right)\varrho_{\max}^2T \\
        &\quad+ \frac{8\eta^2l_{g,1}^2I^2}{\lambda^2\mu^2}\left(1 + \frac{72l_{g,1}^2L^2}{\lambda^2\mu^2}\left(\frac{\eta^2}{\nu^2} + \eta^2I^2\right)\right)\sum_{t=1}^{\tau-1}\left(\|\gdphi(x_t)\|^2 + \|\epsilon_t\|^2\right) \\
        &\quad+ \frac{8\eta^2l_{g,1}^2I^2}{\lambda^2\mu^2}\left(1 + \frac{72l_{g,1}^2L^2}{\lambda^2\mu^2}\left(\frac{\eta^2}{\nu^2} + \eta^2I^2\right)\right)\frac{l_{g,1}^2l_{f,0}^2}{\mu^2}\left(1-\frac{\mu}{l_{g,1}}\right)^{2Q},
    \end{aligned}
\end{equation*}
where the first inequality uses \eqref{eq:vr-yt-and-mi-sum}, the third inequality is due to Young's inequality, and the last inequality uses \eqref{eq:vr-haty-sum}.
\end{proof}

%%%%%%%%%%%%%%%%%%%%%%%%%%%%%%%%%%%%%%%%%%%%%%%%%%%%%%%%%%%%%%%%%%%%%%%%%%%%%%%%%%%%%%%%%%%%%%%
The next lemma is a generalization of \citep[Lemma D.4]{li2023convergence} under the bilevel optimization setting.

\begin{lemma} \label{lm:Wt-bound}
Under the parameter choices in \cref{thm:vr-main-appendix}, if $t\leq \tau$, and $\eta, \nu, I, \varrho_{\max}, \hrho_{\max}$ further satisfy
\begin{equation} \label{eq:Wt-rs-condition}
    \begin{aligned}
        \left(\left(1+\frac{\nu l_{g,1}}{\mu}\right)\frac{\eta}{\lambda} + \frac{\nu\eta l_{g,1}I}{\lambda\mu}\right)\max_{t\leq T}\|m_t\| + \nu(\varrho_{\max} + \hrho_{\max}) \leq r,
        \quad
        \hrho_{\max} \coloneqq \max_{t\leq T}\|\hy_t-y_t^*\| \leq r,
        % \quad\text{where}\quad
        % \hrho_{\max}\coloneqq \max_{t\leq T}\|\hy_t-y_t^*\|,
    \end{aligned}
\end{equation}
then we have
\begin{equation*}
    \begin{aligned}
        \|W_t\| 
        &\leq \beta\sigma_{\phi} + \frac{2\eta L}{\lambda}\left(1+\frac{\nu l_{g,1}}{\mu}\right)(\|\gdphi(x_{t-1})\| + \|\epsilon_{t-1}\|) + \left(2\nu L + \frac{2\eta L^2}{\lambda}\left(1+\frac{\nu l_{g,1}}{\mu}\right)\right)\|\hy_{t-1}-y_{t-1}^*\| \\
        &\quad+ 2\nu L\|y_t-y_t^*\| + \frac{2\eta Ll_{g,1}l_{f,0}}{\lambda\mu}\left(1+\frac{\nu l_{g,1}}{\mu}\right)\left(1-\frac{\mu}{l_{g,1}}\right)^Q.
    \end{aligned}
\end{equation*}
\end{lemma}

\begin{proof}[Proof of \cref{lm:Wt-bound}]
By the definition of $W_t$, we know that
\begin{equation*}
    \begin{aligned}
        W_t = \beta(\hatphi(x_t,\hy_t;\Bar{\xi}_t) - \E_t[\hatphi(x_t,\hy_t;\Bar{\xi}_t)]) + (1-\beta)\delta_t, 
    \end{aligned}
\end{equation*}
where $\delta_t$ is denoted as
\begin{equation*}
    \begin{aligned}
        \delta_t = \hatphi(x_t,\hy_t;\Bar{\xi}_t) - \hatphi(x_{t-1},\hy_{t-1};\Bar{\xi}_t) - \E_t[\hatphi(x_t,\hy_t;\Bar{\xi}_t)] + \E_t[\hatphi(x_{t-1},\hy_{t-1};\Bar{\xi}_t)].
    \end{aligned}
\end{equation*}
By condition \eqref{eq:Wt-rs-condition} and \cref{lm:vr-yt-max-error}, it is easy to verify that
\begin{equation*}
    \begin{aligned}
        \|x_t-x_{t-1}\| + \|\hy_t-\hy_{t-1}\|
        &\leq \left(1+\frac{\nu l_{g,1}}{\mu}\right)\frac{\eta}{\lambda}\|m_{t-1}\| + \nu\|y_t-y_t^*\| + \nu\|\hy_{t-1}-y_{t-1}^*\| \\
        &\leq \left(1+\frac{\nu l_{g,1}}{\mu}\right)\frac{\eta}{\lambda}\max_{t\leq T}\|m_t\| + \nu\left(\varrho_{\max}+\frac{\eta l_{g,1}I}{\lambda\mu}\max_{t\leq T}\|m_t\|\right) + \nu\hrho_{\max} \\
        &\leq r.
    \end{aligned}
\end{equation*}
Then we have
\begin{equation*}
    \begin{aligned}
        \|\delta_t\|
        &\leq \|\hatphi(x_t,\hy_t;\Bar{\xi}_t) - \hatphi(x_{t-1},\hy_{t-1};\Bar{\xi}_t)\| + \|\E_t[\hatphi(x_t,\hy_t;\Bar{\xi}_t)] - \E_t[\hatphi(x_{t-1},\hy_{t-1};\Bar{\xi}_t)]\| \\
        &\leq 2L(\|x_t-x_{t-1}\| + \|\hy_t-\hy_{t-1}\|) \\
        &\leq 2L\left(\left(1+\frac{\nu l_{g,1}}{\mu}\right)\|x_t-x_{t-1}\| + \nu\|y_t-y_t^*\| + \nu\|\hy_{t-1}-y_{t-1}^*\|\right) \\
        &\leq 2L\left(\left(1+\frac{\nu l_{g,1}}{\mu}\right)\frac{\eta}{\lambda}\|m_{t-1}\| + \nu\|y_t-y_t^*\| + \nu\|\hy_{t-1}-y_{t-1}^*\|\right) \\
        &\leq \frac{2\eta L}{\lambda}\left(1+\frac{\nu l_{g,1}}{\mu}\right)\left(\|\gdphi(x_{t-1})\| + \|\epsilon_{t-1}\| + L\|\hy_{t-1}-y_{t-1}^*\| + \frac{l_{g,1}l_{f,0}}{\mu}\left(1-\frac{\mu}{l_{g,1}}\right)^Q\right) \\
        &\quad+ 2\nu L(\|y_t-y_t^*\| + \|\hy_{t-1}-y_{t-1}^*\|) \\
        &= \frac{2\eta L}{\lambda}\left(1+\frac{\nu l_{g,1}}{\mu}\right)(\|\gdphi(x_{t-1})\| + \|\epsilon_{t-1}\|) + \left(2\nu L + \frac{2\eta L^2}{\lambda}\left(1+\frac{\nu l_{g,1}}{\mu}\right)\right)\|\hy_{t-1}-y_{t-1}^*\| \\
        &\quad+ 2\nu L\|y_t-y_t^*\| + \frac{2\eta Ll_{g,1}l_{f,0}}{\lambda\mu}\left(1+\frac{\nu l_{g,1}}{\mu}\right)\left(1-\frac{\mu}{l_{g,1}}\right)^Q,
    \end{aligned}
\end{equation*}
where the second inequality uses \cref{lm:hyper-stoc-bias}; the third inequality is due to
\begin{equation*}
    \begin{aligned}
        \|\hy_t-\hy_{t-1}\|
        &\leq \nu\|y_t-y_t^*\| + \nu\|y_t^*-y_{t-1}^*\| + \nu\|y_{t-1}^*-\hy_{t-1}\| \\
        &\leq \frac{\nu l_{g,1}}{\mu}\|x_t-x_{t-1}\| + \nu\|y_t-y_t^*\| + \nu\|y_{t-1}^*-\hy_{t-1}\|;
    \end{aligned}
\end{equation*}
the fourth inequality uses the update rule in \cref{alg:vradambo} and $h_t\preceq\eta/\lambda$ by \cref{lm:vr-terms-bound}; the last inequality is again due to \cref{lm:vr-terms-bound}. Thus we obtain
\begin{equation*}
    \begin{aligned}
        \|W_t\| 
        &\leq \beta\sigma_{\phi} + \frac{2\eta L}{\lambda}\left(1+\frac{\nu l_{g,1}}{\mu}\right)(\|\gdphi(x_{t-1})\| + \|\epsilon_{t-1}\|) + \left(2\nu L + \frac{2\eta L^2}{\lambda}\left(1+\frac{\nu l_{g,1}}{\mu}\right)\right)\|\hy_{t-1}-y_{t-1}^*\| \\
        &\quad+ 2\nu L\|y_t-y_t^*\| + \frac{2\eta Ll_{g,1}l_{f,0}}{\lambda\mu}\left(1+\frac{\nu l_{g,1}}{\mu}\right)\left(1-\frac{\mu}{l_{g,1}}\right)^Q.
    \end{aligned}
\end{equation*}
\end{proof}

%%%%%%%%%%%%%%%%%%%%%%%%%%%%%%%%%%%%%%%%%%%%%%%%%%%%%%%%%%%%%%%%%%%%%%%%%%%%%%%%%%%%%%%%%%%%%%%
The following is the descent lemma for VR-AdamBO, whose proof is similar to that of \cref{lm:descent-lemma}.

\begin{lemma} \label{lm:vr-descent}
Under the parameter choices in \cref{thm:vr-main-appendix}, if $t<\tau$, and $\eta,\hrho_{\max}$ further satisfy
% \begin{equation*}
%     \hrho_{\max} \leq \min\left\{r, \frac{1}{4L_1}\right\},
%     \quad
%     G \geq \max\left\{4C_{\phi,0}, \frac{C_{\phi,1}}{L_1}, 4\lambda\right\},
%     % \quad\quad\text{and}\quad\quad
%     \quad
%     \eta \leq \min\left\{\frac{r\lambda}{\max_{t\leq T}\|m_t\|}, \frac{\lambda}{6L}\right\},
% \end{equation*}
\begin{equation} \label{eq:vr-eta-additional}
    \begin{aligned}
        \eta \leq \frac{r\lambda}{\max_{t\leq T}\|m_t\|}, 
        \quad
        \hrho_{\max} \leq \min\left\{r, \frac{1}{4L_1}\right\},
    \end{aligned}
\end{equation}
then we have
\begin{equation}
    \begin{aligned}
        \Phi(x_{t+1}) - \Phi(x_t) 
        &\leq -\frac{\eta}{4G}\|\gdphi(x_t)\|^2 + \frac{2\eta}{\lambda}\|\epsilon_t\|^2 + \frac{4\eta L^2}{\lambda}\|\hy_t-y_t^*\|^2 \\
        &\quad + \frac{4\eta}{\lambda}\|\E_t[\hatphi(x_t,y_t^*;\Bar{\xi}_t)]-\gdphi(x_t)\|^2.
    \end{aligned}
\end{equation}
\end{lemma}

\begin{proof}[Proof of \cref{lm:vr-descent}]
The proof is essentially the same as that of \cref{lm:descent-lemma}, except for the last step. 
Define $\hat{\epsilon}_t$ and $\epsilon_t$ as
\begin{equation} \label{eq:vr-epsilont-def}
    \hat{\epsilon}_t = m_t-\gdphi(x_t)
    \quad\quad\text{and}\quad\quad
    \epsilon_t = m_t-\E_t[\hatphi(x_t,\hy_t;\Bar{\xi}_t)].
\end{equation}
By choice of $\eta$ in \eqref{eq:vr-eta-additional}, we have
\begin{equation*}
    \|x_{t+1} - x_t\| \leq \frac{\eta}{\lambda}\|m_t\| \leq \frac{r\lambda}{\lambda\max_{t\leq T}\|m_t\|}\|m_t\| \leq r.
\end{equation*}
Then for any $t< \tau$, by \cref{lm:descent-lemma} we have
\begin{equation*}
    \begin{aligned}
        \Phi(x_{t+1}) - \Phi(x_t)
        &\leq -\frac{\eta}{4G}\|\gdphi(x_t)\|^2 + \frac{\eta}{\lambda}\|\hat{\epsilon}_t\|^2 \\
        &\leq -\frac{\eta}{4G}\|\gdphi(x_t)\|^2 + \frac{2\eta}{\lambda}\|\epsilon_t\|^2 + \frac{4\eta}{\lambda}\|\E_t[\hatphi(x_t,\hy_t;\Bar{\xi}_t)] - \E_t[\hatphi(x_t,y_t^*;\Bar{\xi}_t)]\|^2 \\
        &\quad+ \frac{4\eta}{\lambda}\|\E_t[\hatphi(x_t,y_t^*;\Bar{\xi}_t)]-\gdphi(x_t)\|^2 \\
        &\leq -\frac{\eta}{4G}\|\gdphi(x_t)\|^2 + \frac{2\eta}{\lambda}\|\epsilon_t\|^2 + \frac{4\eta L^2}{\lambda}\|\hy_t-y_t^*\|^2 \\
        &\quad + \frac{4\eta}{\lambda}\|\E_t[\hatphi(x_t,y_t^*;\Bar{\xi}_t)]-\gdphi(x_t)\|^2,
    \end{aligned}
\end{equation*}
where the second inequality uses \eqref{eq:vr-epsilont-def} and Young's inequality, the third inequality is due to \cref{lm:hyper-stoc-bias} and the definition of $\nu$.
\end{proof}

%%%%%%%%%%%%%%%%%%%%%%%%%%%%%%%%%%%%%%%%%%%%%%%%%%%%%%%%%%%%%%%%%%%%%%%%%%%%%%%%%%%%%%%%%%%%%%%
The next lemma uses Optional Stopping Theorem () to bound the sum of the error terms $\|\epsilon_t\|^2$ before time $\tau$ in expectation.

\begin{lemma} \label{lm:vr-momentum-error-sum}
Under the parameter choices in \cref{thm:vr-main-appendix}, if $\eta, \nu, I, \varrho_{\max}, \hrho_{\max}$ further satisfy \eqref{eq:Wt-rs-condition} and \eqref{eq:vr-eta-additional},
% \begin{equation*}
%     \eta \leq \frac{r\lambda}{\max_{t\leq T}\|m_t\|}, 
% \end{equation*}
% If $G, S_1, \eta, \nu, \hrho_{\max}$ satisfy
% \begin{equation*}
%     G \geq \max\{2\sigma_{\phi}, 2\lambda\}, 
%     \quad
%     \eta \leq \min\left\{\frac{r\lambda}{\max_{t\leq T}\|m_t\|}, \frac{\mu\lambda^{3/2}}{40L(\mu+l_{g,1})}\sqrt{\frac{\beta}{G}}\right\},
% \end{equation*}
% \begin{equation*}
%     \nu = a_1\sqrt{\beta},
%     \quad
%     I = \frac{a_2}{\sqrt{\beta}},
%     \quad
%     S_1 \geq \frac{1}{2\beta^2T}, 
% \end{equation*}
% \begin{equation*}
%     \begin{aligned}
%         \frac{72\cdot48l_{g,1}^2L^2}{\lambda^2\mu^2}\left(1+a_1^2a_2^2+\left(\frac{1}{a_1^2}+a_2^2\right)\frac{\lambda}{400G}\right)\eta^2 \leq \frac{\lambda\beta}{64G},
%     \end{aligned}
% \end{equation*}
% \begin{equation*}
%     \begin{aligned}
%         \frac{192l_{g,1}^2L^2}{\lambda^2\mu^2}a_1^2a_2^2\eta^2\left(1 + \frac{72l_{g,1}^2L^2}{\lambda^2\mu^2}\left(\frac{1}{a_1^2}+a_2^2\right)\frac{\eta^2}{\beta}\right) \leq \frac{\lambda\beta}{64G},
%     \end{aligned}
% \end{equation*}
% \begin{equation*}
%     \eta \leq \frac{r\lambda}{\max_{t\leq T}\|m_t\|}, 
%     \quad
%     \left(\left(1+\frac{\nu l_{g,1}}{\mu}\right)\frac{\eta}{\lambda} + \frac{\nu\eta l_{g,1}I}{\lambda\mu}\right)\max_{t\leq T}\|m_t\| + \nu(\varrho_{\max} + \hrho_{\max}) \leq r,
%     \quad
%     \hrho_{\max} \leq r,
% \end{equation*}
then we have
\begin{equation*}
    \begin{aligned}
        &\E\left[\sum_{t=1}^{\tau-1}\frac{3\beta}{4}\|\epsilon_t\|^2 - \frac{3\lambda\beta}{64G}\|\gdphi(x_t)\|^2\right] \\
        &\quad\leq 8\beta^2\sigma_{\phi}^2T - \E[\|\epsilon_{\tau}\|^2] + 48L^2\left(\nu^2 + \frac{\lambda\beta}{400G}\right)\left(\frac{6}{\nu}\|\hy_1-y_0^*\|^2 + 12\varrho_{\max}^2T\right) \\
        &\quad\quad+ 24\nu^2L^2\left(\frac{48\eta^2l_{g,1}^2I^2L^2}{\nu\lambda^2\mu^2}\|\hy_1-y_0^*\|^2 + \left(2 + \frac{96\eta^2l_{g,1}^2I^2L^2}{\lambda^2\mu^2}\right)\varrho_{\max}^2T\right) \\
        &\quad\quad+ \left(\frac{\lambda\beta}{32G} + \frac{24\eta^2L^2T}{\lambda^2}\left(1+\frac{l_{g,1}}{\mu}\right)^2\right)\frac{l_{g,1}^2l_{f,0}^2}{\mu^2}\left(1-\frac{\mu}{l_{g,1}}\right)^{2Q},
    \end{aligned}
\end{equation*}
\end{lemma}

\begin{proof}[Proof of \cref{lm:vr-momentum-error-sum}]
By \cref{lm:Wt-bound} we have
\begin{equation*}
    \begin{aligned}
        \|W_t\|^2
        &\leq 6\beta^2\sigma_{\phi}^2 + \frac{24\eta^2L^2}{\lambda^2}\left(1+\frac{\nu l_{g,1}}{\mu}\right)^2(\|\gdphi(x_{t-1})\|^2 + \|\epsilon_{t-1}\|^2) \\
        &\quad+ 6\left(2\nu L + \frac{2\eta L^2}{\lambda}\left(1+\frac{\nu l_{g,1}}{\mu}\right)\right)^2\|\hy_{t-1}-y_{t-1}^*\|^2 + 24\nu^2L^2\|y_t-y_t\|^2 \\
        &\quad+ \frac{24\eta^2L^2l_{g,1}^2l_{f,0}^2}{\lambda^2\mu^2}\left(1+\frac{\nu l_{g,1}}{\mu}\right)^2\left(1-\frac{\mu}{l_{g,1}}\right)^{2Q} \\
        &\leq 6\beta^2\sigma_{\phi}^2 + \frac{\lambda\beta}{64G}(\|\gdphi(x_{t-1})\|^2 + \|\epsilon_{t-1}\|^2) + 48L^2\left(\nu^2 + \frac{\lambda\beta}{400G}\right)\|\hy_{t-1}-y_{t-1}^*\|^2 \\
        &\quad+ 24\nu^2L^2\|y_t-y_t\|^2 + \frac{24\eta^2L^2l_{g,1}^2l_{f,0}^2}{\lambda^2\mu^2}\left(1+\frac{l_{g,1}}{\mu}\right)^2\left(1-\frac{\mu}{l_{g,1}}\right)^{2Q} \\
    \end{aligned}
\end{equation*}
where the first inequality uses Young's inequality; the second inequality is due to \cref{lm:sum-hy-and-y}, $\nu<1$ and choices of $\eta,\beta$ such that
\begin{equation*}
    \eta = \frac{\sigma_{g,1}\sqrt{\beta}}{\sqrt{C_2}\mu} \leq \frac{\mu\lambda^{3/2}}{40L(\mu+l_{g,1})}\sqrt{\frac{\beta}{G}},
\end{equation*}
where in the last inequality we choose large enough $C_2$.
Note that
\begin{equation*}
    \begin{aligned}
        \|\epsilon_t\|
        &= (1-\beta)^2\|\epsilon_{t-1}\|^2 + \|W_t\|^2 + (1-\beta)\langle \epsilon_{t-1}, W_t \rangle.
    \end{aligned}
\end{equation*}
Taking summation over $2\leq t\leq \tau$, we obtain
\begin{equation*}
    \begin{aligned}
        \sum_{t=2}^{\tau}\|\epsilon_t\|^2
        &\leq (1-\beta)^2\sum_{t=2}^{\tau}\|\epsilon_{t-1}\|^2 + \sum_{t=2}^{\tau}\|W_t\|^2 + (1-\beta)\sum_{t=2}^{\tau}\langle \epsilon_{t-1}, W_t \rangle \\
        &\leq (1-\beta)^2\sum_{t=2}^{\tau}\|\epsilon_{t-1}\|^2 + (1-\beta)\sum_{t=2}^{\tau}\langle \epsilon_{t-1}, W_t \rangle \\
        &\quad+ 6\beta^2\sigma_{\phi}^2(\nu-1) + \frac{\lambda\beta}{64G}\sum_{t=2}^{\tau}\|\gdphi(x_{t-1})\|^2 + \|\epsilon_{t-1}\|^2 \\
        &\quad+ 48L^2\left(\nu^2 + \frac{\lambda\beta}{400G}\right)\sum_{t=2}^{\tau}\|\hy_{t-1}-y_{t-1}^*\|^2 + 24\nu^2L^2\sum_{t=2}^{\tau}\|y_t-y_t\|^2 \\
        &\quad + \frac{24\eta^2L^2l_{g,1}^2l_{f,0}^2(\nu-1)}{\lambda^2\mu^2}\left(1+\frac{l_{g,1}}{\mu}\right)^2\left(1-\frac{\mu}{l_{g,1}}\right)^{2Q} \\
        &\leq (1-\beta)^2\sum_{t=2}^{\tau}\|\epsilon_{t-1}\|^2 + \frac{3\lambda\beta}{64G}\sum_{t=2}^{\tau}(\|\gdphi(x_{t-1})\|^2 + \|\epsilon_{t-1}\|^2) + (1-\beta)\sum_{t=2}^{\tau}\langle \epsilon_{t-1}, W_t \rangle \\
        &\quad+ 6\beta^2\sigma_{\phi}^2T + 48L^2\left(\nu^2 + \frac{\lambda\beta}{400G}\right)\left(\frac{6}{\nu}\|\hy_1-y_0^*\|^2 + 12\varrho_{\max}^2T\right) \\
        &\quad+ 24\nu^2L^2\left(\frac{48\eta^2l_{g,1}^2I^2L^2}{\nu\lambda^2\mu^2}\|\hy_1-y_0^*\|^2 + \left(2 + \frac{96\eta^2l_{g,1}^2I^2L^2}{\lambda^2\mu^2}\right)\varrho_{\max}^2T\right) \\
        &\quad+ \left(\frac{\lambda\beta}{32G} + \frac{24\eta^2L^2T}{\lambda^2}\left(1+\frac{l_{g,1}}{\mu}\right)^2\right)\frac{l_{g,1}^2l_{f,0}^2}{\mu^2}\left(1-\frac{\mu}{l_{g,1}}\right)^{2Q} \\
        &\leq (1-3\beta/4)\sum_{t=2}^{\tau}\|\epsilon_{t-1}\|^2 + \frac{3\lambda\beta}{64G}\sum_{t=2}^{\tau}\|\gdphi(x_{t-1})\|^2 + (1-\beta)\sum_{t=2}^{\tau}\langle \epsilon_{t-1}, W_t \rangle \\
        &\quad+ 6\beta^2\sigma_{\phi}^2T + 48L^2\left(\nu^2 + \frac{\lambda\beta}{400G}\right)\left(\frac{6}{\nu}\|\hy_1-y_0^*\|^2 + 12\varrho_{\max}^2T\right) \\
        &\quad+ 24\nu^2L^2\left(\frac{48\eta^2l_{g,1}^2I^2L^2}{\nu\lambda^2\mu^2}\|\hy_1-y_0^*\|^2 + \left(2 + \frac{96\eta^2l_{g,1}^2I^2L^2}{\lambda^2\mu^2}\right)\varrho_{\max}^2T\right) \\
        &\quad+ \left(\frac{\lambda\beta}{32G} + \frac{24\eta^2L^2T}{\lambda^2}\left(1+\frac{l_{g,1}}{\mu}\right)^2\right)\frac{l_{g,1}^2l_{f,0}^2}{\mu^2}\left(1-\frac{\mu}{l_{g,1}}\right)^{2Q},
    \end{aligned}
\end{equation*}
where the third inequality uses \cref{lm:sum-hy-and-y} and the choices of $\eta$ and $\beta$, and the last inequality is due to $G\geq \lambda$. Taking expectations on both sides, rearranging the terms, and noting that
\begin{equation*}
    \begin{aligned}
        \E\left[\sum_{t=2}^{\tau}\langle \epsilon_{t-1}, W_t \rangle\right] = 0
    \end{aligned}
\end{equation*}
by the Optional Stopping Theorem (i.e., \cref{lm:optional-stopping-thm}), we have
\begin{equation*}
    \begin{aligned}
        &\E\left[\sum_{t=1}^{\tau-1}\frac{3\beta}{4}\|\epsilon_t\|^2 - \frac{3\lambda\beta}{64G}\|\gdphi(x_t)\|^2\right] \\
        &\quad\leq 8\beta^2\sigma_{\phi}^2T - \E[\|\epsilon_{\tau}\|^2] + 48L^2\left(\nu^2 + \frac{\lambda\beta}{400G}\right)\left(\frac{6}{\nu}\|\hy_1-y_0^*\|^2 + 12\varrho_{\max}^2T\right) \\
        &\quad\quad+ 24\nu^2L^2\left(\frac{48\eta^2l_{g,1}^2I^2L^2}{\nu\lambda^2\mu^2}\|\hy_1-y_0^*\|^2 + \left(2 + \frac{96\eta^2l_{g,1}^2I^2L^2}{\lambda^2\mu^2}\right)\varrho_{\max}^2T\right) \\
        &\quad\quad+ \left(\frac{\lambda\beta}{32G} + \frac{24\eta^2L^2T}{\lambda^2}\left(1+\frac{l_{g,1}}{\mu}\right)^2\right)\frac{l_{g,1}^2l_{f,0}^2}{\mu^2}\left(1-\frac{\mu}{l_{g,1}}\right)^{2Q},
    \end{aligned}
\end{equation*}
where the inequality uses the choice of $S_1$ to derive $\E[\|\epsilon_1\|]\leq \sigma_{\phi}^2/S_1 \leq 2\beta^2\sigma_{\phi}^2T$.
\end{proof}

%%%%%%%%%%%%%%%%%%%%%%%%%%%%%%%%%%%%%%%%%%%%%%%%%%%%%%%%%%%%%%%%%%%%%%%%%%%%%%%%%%%%%%%%%%%%%%%
Combing \cref{lm:vr-descent,lm:vr-momentum-error-sum}, we obtain the following lemma.

\begin{lemma} \label{lm:vr-three-bounds}
% Under the parameter settings in \cref{lm:vr-descent,lm:vr-momentum-error-sum}, if $\eta,\beta$ further satisfy
% \begin{equation*}
%     \begin{aligned}
%         % \frac{32GL^2}{\lambda}\frac{72l_{g,1}^2L^2}{\lambda^2\mu^2}\left(\frac{1}{a_1^2}+a_2^2\right)\frac{\eta^2}{\beta} \leq \min\left\{\frac{4G}{\lambda}, \frac{1}{4}\right\},
%         \frac{32\cdot72Gl_{g,1}^2L^2}{\lambda^3\mu^2}\left(\frac{1}{a_1^2}+a_2^2\right)\frac{\eta^2}{\beta} \leq \min\left\{\frac{4G}{\lambda}, \frac{1}{4}\right\},
%     \end{aligned}
% \end{equation*}
Under the parameter choices in \cref{thm:vr-main-appendix}, if $\eta, \nu, I, \varrho_{\max}, \hrho_{\max}$ further satisfy \eqref{eq:Wt-rs-condition} and \eqref{eq:vr-eta-additional}, then we have
\begin{equation*}
    \begin{aligned}
        \E\left[\sum_{t=1}^{\tau-1}\|\gdphi(x_t)\|^2\right] \leq \gI,
        \quad
        \E[\Phi(x_{\nu}) - \Phi^*] \leq \frac{\eta\gI}{8G}, 
        \quad
        \E[\|\epsilon_{\tau}\|^2] \leq \frac{\lambda\beta\gI}{16G},
    \end{aligned}
\end{equation*}
where $\gI$ is defined in \eqref{eq:mathcal-I-def}.
\end{lemma}

\begin{proof}[Proof of \cref{lm:vr-three-bounds}]
By \cref{lm:vr-descent}, if $t<\tau$, then
\begin{equation*}
    \begin{aligned}
        \Phi(x_{t+1}) - \Phi(x_t) 
        &\leq -\frac{\eta}{4G}\|\gdphi(x_t)\|^2 + \frac{2\eta}{\lambda}\|\epsilon_t\|^2 + \frac{4\eta L^2}{\lambda}\|\hy_t-y_t^*\|^2 \\
        &\quad + \frac{4\eta}{\lambda}\|\E_t[\hatphi(x_t,y_t^*;\Bar{\xi}_t)]-\gdphi(x_t)\|^2.
    \end{aligned}
\end{equation*}
Taking summation over $1\leq t< \tau$, rearranging terms, multiplying both sides by $8G/\eta$, and taking expectation, we obtain
\begin{equation} \label{eq:vr-final-sum-1}
    \begin{aligned}
        &\E\left[\sum_{t=1}^{\tau-1}2\|\gdphi(x_t)\|^2 - \frac{8G}{\eta}\|\epsilon_t\|^2\right] \\
        &\leq \frac{8G}{\eta}\E[\Phi(x_1)-\Phi(x_{\nu})] + \frac{32GL^2}{\lambda}\E\left[\sum_{t=1}^{\tau-1}\|\hy_t-y_t^*\|^2\right]
        + \frac{32GTl_{g,1}^2l_{f,0}^2}{\lambda\mu^2}\left(1-\frac{\mu}{l_{g,1}}\right)^{2Q} \\
        &\leq \frac{8G}{\eta}\E[\Phi(x_1)-\Phi(x_{\nu})] + \frac{32GL^2}{\lambda}\left(\frac{6}{\nu}\|\hy_1-y_0^*\|^2 + 12\varrho_{\max}^2T\right) \\
        &\quad+ \frac{32\cdot72Gl_{g,1}^2L^2}{\lambda^3\mu^2}\left(\frac{\eta^2}{\nu^2} + \eta^2I^2\right)\E\left[\sum_{t=1}^{\tau-1}\|\gdphi(x_t)\|^2 + \|\epsilon_t\|^2\right] \\
        &\quad+ \left(\frac{32GT}{\lambda} + \frac{32\cdot72GTl_{g,1}^2L^2}{\lambda^3\mu^2}\left(\frac{\eta^2}{\nu^2} + \eta^2I^2\right)\right)\frac{l_{g,1}^2l_{f,0}^2}{\mu^2}\left(1-\frac{\mu}{l_{g,1}}\right)^{2Q} \\
        &\leq \frac{8G}{\eta}\E[\Phi(x_1)-\Phi(x_{\nu})] + \frac{32GL^2}{\lambda}\left(\frac{6}{\nu}\|\hy_1-y_0^*\|^2 + 12\varrho_{\max}^2T\right) \\
        &\quad+ \E\left[\sum_{t=1}^{\tau-1}\frac{1}{4}\|\gdphi(x_t)\|^2 + \frac{4G}{\lambda}\|\epsilon_t\|^2\right] 
        + \left(\frac{32GT}{\lambda} + \frac{32\cdot72GTl_{g,1}^2L^2}{\lambda^3\mu^2}\left(\frac{\eta^2}{\nu^2} + \eta^2I^2\right)\right)\frac{l_{g,1}^2l_{f,0}^2}{\mu^2}\left(1-\frac{\mu}{l_{g,1}}\right)^{2Q},
    \end{aligned}
\end{equation}
where the second inequality uses \cref{lm:sum-hy-and-y}, and the last inequality is due to the choices of $\eta$ and $\beta$. Also, by \cref{lm:vr-momentum-error-sum} we have
\begin{equation} \label{eq:vr-final-sum-2}
    \begin{aligned}
        &\E\left[\sum_{t=1}^{\tau-1}\frac{12G}{\lambda}\|\epsilon_t\|^2 - \frac{3}{4}\|\gdphi(x_t)\|^2\right] \\
        &\quad\leq \frac{128G\sigma_{\phi}^2\beta T}{\lambda} - \frac{16G}{\lambda\beta}\E[\|\epsilon_{\tau}\|^2] + \frac{16\cdot48GL^2}{\lambda\beta}\left(\nu^2 + \frac{\lambda\beta}{400G}\right)\left(\frac{6}{\nu}\|\hy_1-y_0^*\|^2 + 12\varrho_{\max}^2T\right) \\
        &\quad\quad+ \frac{16\cdot24\nu^2GL^2}{\lambda\beta}\left(\frac{48\eta^2l_{g,1}^2I^2L^2}{\nu\lambda^2\mu^2}\|\hy_1-y_0^*\|^2 + \left(2 + \frac{96\eta^2l_{g,1}^2I^2L^2}{\lambda^2\mu^2}\right)\varrho_{\max}^2T\right) \\
        &\quad\quad+ \frac{16G}{\lambda\beta}\left(\frac{\lambda\beta}{32G} + \frac{24\eta^2L^2T}{\lambda^2}\left(1+\frac{l_{g,1}}{\mu}\right)^2\right)\frac{l_{g,1}^2l_{f,0}^2}{\mu^2}\left(1-\frac{\mu}{l_{g,1}}\right)^{2Q}.
    \end{aligned}
\end{equation}
Then summing $\eqref{eq:vr-final-sum-1} + \eqref{eq:vr-final-sum-2}$ gives
\begin{equation} \label{eq:mathcal-I-def}
    \begin{aligned}
        &\E\left[\sum_{t=1}^{\tau-1}\|\gdphi(x_t)\|^2\right] + \frac{8G}{\eta}\E[\Phi(x_{\nu}) - \Phi^*] + \frac{16G}{\lambda\beta}\E[\|\epsilon_{\tau}\|^2] \\
        &\leq \frac{8G\Delta_1}{\eta} + \frac{128G\sigma_{\phi}^2\beta T}{\lambda} + \left(\frac{32GL^2}{\lambda} + \frac{16\cdot48GL^2}{\lambda\beta}\left(\nu^2 + \frac{\lambda\beta}{400G}\right)\right)\left(\frac{6}{\nu}\|\hy_1-y_0^*\|^2 + 12\varrho_{\max}^2T\right) \\
        &\quad+ \frac{16\cdot24\nu^2GL^2}{\lambda\beta}\left(\frac{48\eta^2l_{g,1}^2I^2L^2}{\nu\lambda^2\mu^2}\|\hy_1-y_0^*\|^2 + \left(2 + \frac{96\eta^2l_{g,1}^2I^2L^2}{\lambda^2\mu^2}\right)\varrho_{\max}^2T\right) \\
        &\quad+ \left[\left(\frac{32GT}{\lambda} + \frac{32\cdot72GTl_{g,1}^2L^2}{\lambda^3\mu^2}\left(\frac{\eta^2}{\nu^2} + \eta^2I^2\right)\right) \right.\\
        &\left.\quad+ \frac{16G}{\lambda\beta}\left(\frac{\lambda\beta}{32G} + \frac{24\eta^2L^2T}{\lambda^2}\left(1+\frac{l_{g,1}}{\mu}\right)^2\right)\right]\frac{l_{g,1}^2l_{f,0}^2}{\mu^2}\left(1-\frac{\mu}{l_{g,1}}\right)^{2Q} \\
        &\coloneqq \gI,
    \end{aligned}
\end{equation}
which implies that
\begin{equation*}
    \begin{aligned}
        \E\left[\sum_{t=1}^{\tau-1}\|\gdphi(x_t)\|^2\right] \leq \gI,
        \quad
        \E[\Phi(x_{\nu}) - \Phi^*] \leq \frac{\eta\gI}{8G}, 
        \quad
        \E[\|\epsilon_{\tau}\|^2] \leq \frac{\lambda\beta\gI}{16G}.
    \end{aligned}
\end{equation*}
% If $\nu=\nu_1\leq T$, then by definition of $\nu_1$ we know $\Phi(x_{\nu})-\Phi^* > \psi$, and we have
% \begin{equation*}
%     \begin{aligned}
%         \pr(\nu=\nu_1\leq T)
%         &\leq \pr(\Phi(x_{\nu})-\Phi^* > \psi)
%         \leq \frac{\E[\Phi(x_{\nu})-\Phi^*]}{\psi}
%         \leq \frac{\eta\gI}{8G\psi}
%     \end{aligned}
% \end{equation*}
\end{proof}

%%%%%%%%%%%%%%%%%%%%%%%%%%%%%%%%%%%%%%%%%%%%%%%%%%%%%%%%%%%%%%%%%%%%%%%%%%%%%%%%%%%%%%%%%%%%%%%

\subsection{Lower-Level Error Control}

In this section, we aim to provide high probability bound for the lower-level estimation error. First, we present the following high probability guarantee for SNAG (\cref{alg:snag}), as implied by \citep[Lemmas C.3 and C.6]{gong2024accelerated}.

\begin{lemma}[SNAG] \label{lm:snag}
Suppose that \cref{ass:bilevel-assumption,ass:noise,ass:individual-noise} hold. Let $\{\ty_t\}$ be the iterates generated by \cref{alg:snag} with constant learning rate $\gamma\leq 1/2l_{g,1}$. Then for any given $\delta\in(0,1)$ and any fixed $t\geq 1$, the following holds with probability at least $1-\delta$ over the randomness in $\Tilde{\gF}_{T_0}^{y}$: 
\begin{equation*}
    \begin{aligned}
        \|\ty_t - y^*(\tx)\|^2 \leq \frac{3}{\mu\gamma}\left(1-\frac{\sqrt{\mu\gamma}}{4}\right)^t\|\ty_0-y^*(\tx)\|^2 + \frac{4\gamma\sigma_{g,1}^2}{\mu}\ln\frac{e}{\delta}.
    \end{aligned}
\end{equation*}
\end{lemma}

\begin{proof}[Proof of \cref{lm:snag}]
We will use a short hand $\ty^*=y^*(\tx)$. By \citep[Lemmas C.6 and C.3]{gong2024accelerated}, we have
\begin{equation*}
    \begin{aligned}
        V_t \leq \left(1-\frac{\sqrt{\mu\gamma}}{4}\right)^tV_0 + \frac{4\gamma\sigma_{g,1}^2}{\mu}\ln\frac{eT_0}{\delta},
    \end{aligned}
\end{equation*}
where $V_t$ is the notation defined in \citep[Lemmas C.3]{gong2024accelerated} which satisfy the following by noting that $\ty_{-1}=\ty_0$ and $\mu\gamma\leq 1$:
\begin{equation*}
    V_t \geq \frac{\mu}{2}\|\ty_t-\ty^*\|^2,
    \quad\quad
    V_0 \leq \frac{1+(1-\sqrt{\mu\gamma})^2}{2\gamma}\|\ty_0-\ty^*\|^2 \leq \frac{3}{2\gamma}\|\ty_0-\ty^*\|^2.
\end{equation*}
Therefore, we obtain
\begin{equation*}
    \begin{aligned}
        \frac{\mu}{2}\|\ty_t-\ty^*\|^2 \leq \frac{3}{2\gamma}\left(1-\frac{\sqrt{\mu\gamma}}{4}\right)^t\|\ty_0-\ty^*\|^2 + 2\gamma\sigma_{g,1}^2\ln\frac{eT_0}{\delta}.
    \end{aligned}
\end{equation*}
Rearranging the above inequality yields the result.
\end{proof}

%%%%%%%%%%%%%%%%%%%%%%%%%%%%%%%%%%%%%%%%%%%%%%%%%%%%%%%%%%%%%%%%%%%%%%%%%%%%%%%%%%%%%%%%%%%%%%%

\begin{lemma} \label{lm:first-window}
% Suppose that \cref{ass:bilevel-assumption,ass:noise,ass:individual-noise} hold. 
% Consider \cref{alg:vradambo} for $1\leq t\leq I$. 
Under the parameter choices in \cref{thm:vr-main-appendix}, for any given $\delta\in(0,1)$, the following holds with probability at least $1-I\delta/8T$ over the randomness in $\sigma(\gF_{\init}\cup(\cup_{t\leq T}\gF_{t}^y))$ (we denote this event as $\gE_y$): 
\begin{equation*}
    \begin{aligned}
        \|y_t-y_t^*\| 
        \leq \eta + \frac{\eta l_{g,1}}{\lambda\mu}\sum_{i=k_tI}^{t-1}\|m_i\|,
    \end{aligned}
\end{equation*}
where $k_t=\lfloor t/I \rfloor$ and we define $m_0=0$ for completeness.
\end{lemma}

\begin{proof}[Proof of \cref{lm:first-window}]
By line 3 of \cref{alg:vradambo}, \cref{lm:snag,sec:vr-para-verify}, with probability at least $1-\delta/8T$ over the randomness in $\gF_{\init}$ we have
\begin{equation*}
    \begin{aligned}
        \|y_1-y_0^*\|^2
        \leq \frac{3}{\mu\gamma}\left(1-\frac{\sqrt{\mu\gamma}}{4}\right)^{T_0}\|y_0-y_0^*\|^2 + \frac{4\gamma\sigma_{g,1}^2}{\mu}\ln\frac{8eT}{\delta} 
        \leq \frac{\eta^2}{2} + \frac{\eta^2}{2}
        = \eta^2,
    \end{aligned}
\end{equation*}
which gives $\|y_1-y_0^*\|\leq \eta$. Then for any $1\leq t\leq I$, we have
\begin{equation*}
    \begin{aligned}
        \|y_t-y_t^*\| 
        &\leq \|y_1-y_0^*\| + \sum_{i=0}^{t-1}\|y_i^*-y_{i+1}^*\| 
        % \leq \eta + \sum_{i=0}^{I-1}\|y_i^*-y_{i+1}^*\| \\
        \leq \eta + \sum_{i=0}^{t-1}\|y_i^*-y_{i+1}^*\| \\
        % &\leq \eta + \frac{l_{g,1}}{\mu}\sum_{i=0}^{I-1}\|x_{i+1}-x_i\| 
        &\leq \eta + \frac{l_{g,1}}{\mu}\sum_{i=0}^{t-1}\|x_{i+1}-x_i\| 
        % \leq \eta + \frac{\eta l_{g,1}}{\lambda\mu}\sum_{i=0}^{I-1}\|m_i\|.
        \leq \eta + \frac{\eta l_{g,1}}{\lambda\mu}\sum_{i=0}^{t-1}\|m_i\|.
    \end{aligned}
\end{equation*}
Also, under the parameter choices in \cref{thm:vr-main-appendix}, \cref{lm:general-window} shows that $\|y_{kI+1}-y_{kI}^*\|\leq \eta$ for all $k$. Similarly, for $k_tI+1\leq t\leq (k_t+1)I$ we have
\begin{equation*}
    \begin{aligned}
        \|y_t-y_t^*\| 
        \leq \eta + \frac{\eta l_{g,1}}{\lambda\mu}\sum_{i=k_tI}^{t-1}\|m_i\|.
    \end{aligned}
\end{equation*}
\end{proof}

%%%%%%%%%%%%%%%%%%%%%%%%%%%%%%%%%%%%%%%%%%%%%%%%%%%%%%%%%%%%%%%%%%%%%%%%%%%%%%%%%%%%%%%%%%%%%%%

% \begin{lemma} \label{lm:average}
% Consider the averaging step (line 15) of \cref{alg:vradambo}, we have
% \begin{equation*}
%     \begin{aligned}
%         \|\hy_t-y_t^*\|
%         \leq (1-\nu)^t\|\hy_1-y_0^*\| + \frac{(1-\nu)\eta l_{g,1}}{\lambda\mu}\sum_{i=1}^{t}(1-\nu)^{t-i}\|m_{i-1}\| + \nu\sum_{i=1}^{t}(1-\nu)^{t-i}\|y_i-y_i^*\|.
%     \end{aligned}
% \end{equation*}
% \end{lemma}

% \begin{proof}[Proof of \cref{lm:average}]
% Define $\hy_0=y_0$ for simplicity. By the update rule of $\hy_t$, we have
% \begin{equation*}
%     \begin{aligned}
%         \|\hy_t-y_t^*\|
%         &= \|(1-\nu)(\hy_{t-1}-y_t^*) + \nu(y_t-y_t^*)\| \\
%         &= \|(1-\nu)(\hy_{t-1}-y_{t-1}^*) + (1-\nu)(y_{t-1}^*-y_t^*) + \nu(y_t-y_t^*)\| \\
%         &\leq (1-\nu)\|\hy_{t-1}-y_{t-1}^*\| + (1-\nu)\|y_{t-1}^*-y_t^*\| + \nu\|y_t-y_t^*\|.
%     \end{aligned}
% \end{equation*}
% We apply the above inequality recursively to obtain
% \begin{equation*}
%     \begin{aligned}
%         \|\hy_t-y_t^*\| 
%         &\leq (1-\nu)^t\|\hy_0-y_0^*\| + (1-\nu)\sum_{i=2}^{t}(1-\nu)^{t-i}\|y_{i-1}^*-y_i^*\| + \nu\sum_{i=2}^{t}(1-\nu)^{t-i}\|y_i-y_i^*\| \\
%         &\leq (1-\nu)^t\|\hy_1-y_0^*\| + \frac{(1-\nu)\eta l_{g,1}}{\lambda\mu}\sum_{i=1}^{t}(1-\nu)^{t-i}\|m_{i-1}\| + \nu\sum_{i=1}^{t}(1-\nu)^{t-i}\|y_i-y_i^*\|.
%     \end{aligned}
% \end{equation*}
% \end{proof}

%%%%%%%%%%%%%%%%%%%%%%%%%%%%%%%%%%%%%%%%%%%%%%%%%%%%%%%%%%%%%%%%%%%%%%%%%%%%%%%%%%%%%%%%%%%%%%%

\begin{lemma} \label{lm:first-window-bound}
Consider \cref{alg:vradambo} for $1\leq t\leq I$. 
% Choosing $\eta,\nu,I$ that satisfy
% \begin{equation*}
%     \frac{\eta l_{g,1}L}{\lambda\mu}\left(\frac{1-\nu}{\nu} + I\right) \leq \frac{1}{2}.
% \end{equation*}
Under event $\gE_y$ and the parameter choices in \cref{thm:vr-main-appendix}, if $t\leq \tau$, we have
\begin{equation} \label{eq:vr-average-bias-bound}
    \begin{aligned}
        \|\hy_t-y_t^*\|
        \leq \hrho 
        \coloneqq \left(\|\hy_1-y_0^*\| + \eta + \frac{\eta l_{g,1}}{\lambda\mu}\left(\frac{1-\nu}{\nu} + I\right)\left(2G + \frac{l_{g,1}l_{f,0}}{\mu}\right)\right) \Big/ \left(1-\frac{\eta l_{g,1}L}{\lambda\mu}\left(\frac{1-\nu}{\nu} + I\right)\right);
    \end{aligned}
\end{equation}
if $t<\tau$, we have
\begin{equation} \label{eq:vr-mt-bound}
    \begin{aligned}
        \|m_t\|
        \leq C_{m}
        \coloneqq 2G + \frac{l_{g,1}l_{f,0}}{\mu} + Lr.
    \end{aligned}
\end{equation}
\end{lemma}

\begin{proof}[Proof of \cref{lm:first-window-bound}]
For $0\leq t\leq I$, we will use induction to show that if $t<\tau$, then
\begin{equation*}
    \begin{aligned}
        % \|\hy_t-y_t^*\|
        % &\leq \left(\|\hy_1-y_0^*\| + \eta + \frac{\eta l_{g,1}}{\lambda\mu}\left(\frac{1-\nu}{\nu} + I\right)\left(2G + \frac{l_{g,1}l_{f,0}}{\mu}\right)\right) \Big/ \left(1-\frac{\eta l_{g,1}L}{\lambda\mu}\left(\frac{1-\nu}{\nu} + I\right)\right), \\
        % \|m_t\|
        % &\leq 2G + \frac{l_{g,1}l_{f,0}}{\mu} \\
        % &\quad+ L\left(\|\hy_1-y_0^*\| + \eta + \frac{\eta l_{g,1}}{\lambda\mu}\left(\frac{1-\nu}{\nu} + I\right)\left(2G + \frac{l_{g,1}l_{f,0}}{\mu}\right)\right) \Big/ \left(1-\frac{\eta l_{g,1}L}{\lambda\mu}\left(\frac{1-\nu}{\nu} + I\right)\right).
        \|\hy_t-y_t^*\| \leq \hrho,
        \quad\quad\text{and}\quad\quad
        \|m_t\| \leq C_m.
    \end{aligned}
\end{equation*}

\paragraph{Base Case.}
For $t=1$, it is easy to check that
\begin{equation*}
    \begin{aligned}
        \|\hy_1-y_1^*\| = \|\hy_1-y_0^*\| \leq \hrho,
    \end{aligned}
\end{equation*}
where the first equality uses $x_1=x_0$. Also, since $\hrho\leq r$ and thus $\|\hy_1-y_1^*\|\leq r$ by \cref{sec:vr-para-verify}, then we have
\begin{equation*}
    \begin{aligned}
        \|m_1\|
        &\leq \|m_1-\E_1[\hatphi(x_1,\hy_1;\Bar{\xi}_1)]\| + \|\E_1[\hatphi(x_1,\hy_1;\Bar{\xi}_1)] - \E_1[\hatphi(x_1,y_1^*;\Bar{\xi}_1)]\| \\
        &\quad+ \|\E_1[\hatphi(x_1,y_1^*;\Bar{\xi}_1)] - \gdphi(x_1)\| + \|\gdphi(x_1)\| \\
        &\leq \|\epsilon_1\| + (L_0+L\|\gdphi(x_1)\|)\|\hy_1-y_1^*\| + \frac{l_{g,1}l_{f,0}}{\mu}\left(1-\frac{\mu}{l_{g,1}}\right)^Q + \|\gdphi(x_1)\| \\
        &\leq 2G + \frac{l_{g,1}l_{f,0}}{\mu} + L\hrho 
        \leq 2G + \frac{l_{g,1}l_{f,0}}{\mu} + Lr,
    \end{aligned}
\end{equation*}
where the second inequality uses \cref{lm:hyper-stoc-bias,lm:neumann-error}, the third inequality is due to the induction hypothesis and the definition of $\tau$, and the last inequality again uses $\hrho\leq r$ by \cref{sec:vr-para-verify}.
% \begin{equation*}
%     \begin{aligned}
%         \|\hy_1-y_1^*\|
%         &\leq (1-\nu)\|\hy_1-y_0^*\| + (1-\nu)\|y_0^*-y_1^*\| + \nu\|y_1-y_1^*\| \\
%         &\leq \|\hy_1-y_0^*\| + \frac{(1-\nu)\eta l_{g,1}}{\lambda\mu}\|m_0\| + \nu\left(\eta + \frac{\eta l_{g,1}}{\lambda\mu}\|m_0\|\right) \\
%         &= \|\hy_1-y_0^*\| + \nu\rho,
%     \end{aligned}
% \end{equation*}
% where the first inequality uses \cref{lm:first-window}, and the last equality is due to $m_0=0$.
Thus, the base case $t=0$ holds.

\paragraph{Induction Step.}
Suppose the induction hypothesis holds for $t\leq k-1$ with $k<\tau$, then for $t=k$ we have
\begin{equation*}
    \begin{aligned}
        \|\hy_{k}-y_{k}^*\|
        &\leq (1-\nu)^{k}\|\hy_1-y_0^*\| + \frac{(1-\nu)\eta l_{g,1}}{\lambda\mu}\sum_{i=1}^{k}(1-\nu)^{k-i}\|m_{i-1}\| + \nu\sum_{i=1}^{k}(1-\nu)^{k-i}\|y_i-y_i^*\| \\
        &\leq (1-\nu)^{k}\|\hy_1-y_0^*\| + \frac{(1-\nu)\eta l_{g,1}}{\lambda\mu}\sum_{i=1}^{k}(1-\nu)^{k-i}\|m_{i-1}\| \\
        &\quad+ \nu\sum_{i=1}^{k}(1-\nu)^{k-i}\left(\eta + \frac{\eta l_{g,1}}{\lambda\mu}\sum_{j=0}^{i-1}\|m_j\|\right) \\
        &\leq \left(\|\hy_1-y_0^*\| + \eta + \frac{\eta l_{g,1}}{\lambda\mu}\left(\frac{1-\nu}{\nu} + I\right)\left(2G + \frac{l_{g,1}l_{f,0}}{\mu}\right)\right) \Big/ \left(1-\frac{\eta l_{g,1}L}{\lambda\mu}\left(\frac{1-\nu}{\nu} + I\right)\right)
        = \hrho,
    \end{aligned}
\end{equation*}
where the first inequality uses \cref{lm:average}, the second inequality is due to \cref{lm:first-window} and $k\leq I$, and the last inequality uses the induction hypothesis, the sum of geometric series, and the definition of $\hrho$.
Also, we have
\begin{equation*}
    \begin{aligned}
        \|m_k\|
        &\leq \|m_k-\E_k[\hatphi(x_k,\hy_k;\Bar{\xi}_k)]\| + \|\E_k[\hatphi(x_k,\hy_k;\Bar{\xi}_k)] - \E_k[\hatphi(x_k,y_k^*;\Bar{\xi}_k)]\| \\
        &\quad+ \|\E_k[\hatphi(x_k,y_k^*;\Bar{\xi}_k)] - \gdphi(x_k)\| + \|\gdphi(x_k)\| \\
        &\leq \|\epsilon_k\| + (L_0+L\|\gdphi(x_k)\|)\|\hy_k-y_k^*\| + \frac{l_{g,1}l_{f,0}}{\mu}\left(1-\frac{\mu}{l_{g,1}}\right)^Q + \|\gdphi(x_k)\| \\
        &\leq 2G + \frac{l_{g,1}l_{f,0}}{\mu} + L\hrho 
        \leq 2G + \frac{l_{g,1}l_{f,0}}{\mu} + Lr,
    \end{aligned}
\end{equation*}
where the second inequality uses \cref{lm:hyper-stoc-bias,lm:neumann-error}, the third inequality is due to the induction hypothesis and the definition of $\tau$, and the last inequality again uses $\hrho\leq r$ by \cref{sec:vr-para-verify}. Therefore, the induction step is complete. 

% \paragraph{Final Bound.}
% With $\eta,\nu, I$ satisfying 
% \begin{equation*}
%     \frac{\eta l_{g,1}L}{\lambda\mu}\left(\frac{1-\nu}{\nu} + I\right) \leq \frac{1}{2},
% \end{equation*}
% if $t\leq \tau$, we have
% \begin{equation*}
%     \begin{aligned}
%         \|\hy_t-y_t^*\|
%         &\leq \left(\|\hy_1-y_0^*\| + \eta + \frac{\eta l_{g,1}}{\lambda\mu}\left(\frac{1-\nu}{\nu} + I\right)\left(G + \frac{l_{g,1}l_{f,0}}{\mu}\right)\right) \Big/ \left(1-\frac{\eta l_{g,1}L}{\lambda\mu}\left(\frac{1-\nu}{\nu} + I\right)\right) \\
%         &\leq 2\left(\|\hy_1-y_0^*\| + \eta + \frac{1}{2L}\left(G + \frac{l_{g,1}l_{f,0}}{\mu}\right)\right)
%         = \hrho;
%     \end{aligned}
% \end{equation*}
% if $t<\tau$, we have
% \begin{equation*}
%     \begin{aligned}
%         \|m_t\|
%         &\leq \|\epsilon_t\| + L\|\hy_t-y_t^*\| + \frac{l_{g,1}l_{f,0}}{\mu} 
%         \leq G + \frac{l_{g,1}l_{f,0}}{\mu} + L\hrho \\
%         &= G + \frac{l_{g,1}l_{f,0}}{\mu} + 2L\|\hy_1-y_0^*\| + 2G + \frac{l_{g,1}l_{f,0}}{\mu}
%         = C_m.
%     \end{aligned}
% \end{equation*}
\end{proof}

%%%%%%%%%%%%%%%%%%%%%%%%%%%%%%%%%%%%%%%%%%%%%%%%%%%%%%%%%%%%%%%%%%%%%%%%%%%%%%%%%%%%%%%%%%%%%%%

\begin{lemma} \label{lm:general-window}
Under event $\gE_y$ and the parameter choices in \cref{thm:vr-main-appendix}, if $t\leq \tau$, then $\|\hy_t-y_t^*\|\leq \hrho$; and if $t<\tau$, then $\|m_t\|\leq C_m$; where $\hrho$ and $C_m$ are defined in \eqref{eq:vr-average-bias-bound} and \eqref{eq:vr-mt-bound}.
\end{lemma}

\begin{proof}[Proof of \cref{lm:general-window}]
By \cref{lm:first-window-bound}, we know that the statement of \cref{lm:general-window} holds true for $0\leq t\leq I$. Now we consider the case for $I+1\leq t\leq 2I$. First, by \cref{lm:first-window} we know that
\begin{equation*}
    \begin{aligned}
        \|y_I-y_I^*\| 
        \leq \eta + \frac{\eta l_{g,1}}{\lambda\mu}\sum_{i=0}^{I-1}\|m_i\| 
        \leq \eta + \frac{\eta l_{g,1}I}{\lambda\mu}C_m.
    \end{aligned}
\end{equation*}
Then by choice of $N$ and \cref{sec:vr-para-verify} we have
\begin{equation*}
    \begin{aligned}
        \|y_{I+1}-y_I^*\|^2
        \leq \frac{3}{\mu\gamma}\left(1-\frac{\sqrt{\mu\gamma}}{4}\right)^{N}\|y_I-y_I^*\|^2 + \frac{4\gamma\sigma_{g,1}^2}{\mu}\ln\frac{8eT}{\delta} 
        \leq \frac{\eta^2}{2} + \frac{\eta^2}{2}
        = \eta^2,
    \end{aligned}
\end{equation*}
which gives $\|y_{I+1}-y_I^*\|\leq \eta$. Now we follow the same procedure as \cref{lm:first-window,lm:first-window-bound} to obtain the result for $I+1\leq t\leq 2I$. For the general case $k_tI+1\leq t\leq \min\{(k_t+1)I, T\}$, where $1\leq k_t\leq \lfloor T/I \rfloor$, we can easily obtain the results by repeating the previous steps.
\end{proof}

%%%%%%%%%%%%%%%%%%%%%%%%%%%%%%%%%%%%%%%%%%%%%%%%%%%%%%%%%%%%%%%%%%%%%%%%%%%%%%%%%%%%%%%%%%%%%%%
With \cref{lm:general-window}, some of the important quantities in \cref{alg:vradambo} are well bounded before time $\tau$.

\begin{lemma} \label{lm:vr-terms-bound}
Under event $\gE_y$ and the parameter choices in \cref{thm:vr-main-appendix}, if $t<\tau$, we have
\begin{equation*}
    \begin{aligned}
        \hv_t \preceq (C_{u,0} + C_{u,1}\hrho)^2,
        \quad
        \frac{\eta}{C_{u,0} + C_{u,1}\hrho + \lambda} \preceq h_t \preceq \frac{\eta}{\lambda},
    \end{aligned}
\end{equation*}
\begin{equation*}
    \begin{aligned}
        \|m_t\|
        \leq \|\gdphi(x_t)\| + \|\epsilon_t\| + L\|\hy_t-y_t^*\| + \frac{l_{g,1}l_{f,0}}{\mu}\left(1-\frac{\mu}{l_{g,1}}\right)^Q 
        \leq C_m;
    \end{aligned}
\end{equation*}
if $t\leq \tau$, we have
\begin{equation*}
    \|\hy_t-y_t^*\| \leq \hrho,
    \quad
    \|\hatphi(x_t,\hy_t;\Bar{\xi}_t) - \E_t[\hatphi(x_t,\hy_t;\Bar{\xi}_t)]\| \leq \sigma_{\phi}.
\end{equation*}
\end{lemma}

\begin{proof}[Proof of \cref{lm:vr-terms-bound}]
Note that if $t<\tau$, by \cref{lm:vr-gradient-bound} we have
\begin{equation*}
    \begin{aligned}
        \|m_t\|
        % &\leq \|m_t-\E_t[\hatphi(x_t,\hy_t;\Bar{\xi}_t)]\| + \|\E_t[\hatphi(x_t,\hy_t;\Bar{\xi}_t)] - \E_t[\hatphi(x_t,y_t^*;\Bar{\xi}_t)]\| \\
        % &\quad+ \|\E_t[\hatphi(x_t,y_t^*;\Bar{\xi}_t)] - \gdphi(x_t)\| + \|\gdphi(x_t)\| \\
        % &\leq \|\gdphi(x_t)\| + \|\epsilon_t\| + (L_0+L_1\|\gdphi(x_t)\|)\|\hy_t-y_t^*\| + \frac{l_{g,1}l_{f,0}}{\mu}\left(1-\frac{\mu}{l_{g,1}}\right)^Q \\
        &\leq \|\gdphi(x_t)\| + \|\epsilon_t\| + L\|\hy_t-y_t^*\| + \frac{l_{g,1}l_{f,0}}{\mu}\left(1-\frac{\mu}{l_{g,1}}\right)^Q \\
        &\leq 2G + L\hrho + \frac{l_{g,1}l_{f,0}}{\mu}
        \leq 2G + Lr + \frac{l_{g,1}l_{f,0}}{\mu}
        = C_m,
    \end{aligned}
\end{equation*}
where the second inequality uses \cref{lm:general-window}, the third inequality is due to $\hrho\leq r$ by \cref{sec:vr-para-verify}, and the last inequality uses the definition of $C_m$. The remaining terms can be bounded in a similar way as \cref{lm:momentum-bound}.
\end{proof}

%%%%%%%%%%%%%%%%%%%%%%%%%%%%%%%%%%%%%%%%%%%%%%%%%%%%%%%%%%%%%%%%%%%%%%%%%%%%%%%%%%%%%%%%%%%%%%%

% \begin{lemma} \label{lm:vr-rs-condition}
% If $t<\tau$, choosing 
% \begin{equation*}
%     % G + \frac{l_{g,1}l_{f,0}}{\mu} + 2L\|\hy_1-y_0^*\| + G + \frac{l_{g,1}l_{f,0}}{\mu}
%     G \geq 2L\|\hy_1-y_0^*\| + \frac{2l_{g,1}l_{f,0}}{\mu},
% \end{equation*}
% we have $\|x_{t+1}-x_t\|\leq \eta D$ where $D\coloneqq 4G/\lambda$.
% \end{lemma}

% \begin{proof}[Proof of \cref{lm:vr-rs-condition}]
% If $t<\tau$, by \cref{lm:vr-terms-bound} and choice of $G$ we have
% \begin{equation} \label{eq:vr-mt-G}
%     \begin{aligned}
%         \|m_t\| \leq C_m = 3G + 2L\|\hy_1-y_0^*\| + \frac{2l_{g,1}l_{f,0}}{\mu} \leq 4G.
%     \end{aligned}
% \end{equation}
% Then we have
% \begin{equation*}
%     \begin{aligned}
%         \|x_{t+1}-x_t\| \leq \frac{\eta}{\lambda}\|m_t\| \leq \frac{4\eta G}{\lambda} = \eta D,
%     \end{aligned}
% \end{equation*}
% where the first inequality uses the update rule in \cref{alg:vradambo} and $h_t\preceq\eta/\lambda$ by \cref{lm:vr-terms-bound}, and the second inequality is due to \eqref{eq:vr-mt-G}.
% \end{proof}

%%%%%%%%%%%%%%%%%%%%%%%%%%%%%%%%%%%%%%%%%%%%%%%%%%%%%%%%%%%%%%%%%%%%%%%%%%%%%%%%%%%%%%%%%%%%%%%
\subsection{Proof of \cref{thm:vr-main}}
With \cref{lm:vr-three-bounds,lm:vr-terms-bound}, we are ready to prove \cref{thm:vr-main-appendix}. Below is the full statement of \cref{thm:vr-main} with detailed parameter choices, where we use $c_1,c_2$ to denote small enough constants and $C_1,C_2$ to denote large enough ones. The definitions of problem-dependent constants $\sigma_{\phi}, C_{\phi,0}, C_{\phi,1}, \Delta_1, L_0, L_1, L, C_m, C_{\eta}$ are provided in \cref{sec:adambo-notations,sec:vradambo-notations}.

\begin{theorem} \label{thm:vr-main-appendix}
Suppose that \cref{ass:bilevel-assumption,ass:noise,ass:individual-noise} hold. Let $G$ be a constant satisfying 
\begin{equation}
    \begin{aligned}
        G \geq \max\left\{4\lambda, 2\sigma_{\phi}, 4C_{\phi,0}, \frac{C_{\phi,1}}{L_1}, \sqrt{\frac{C_1\Delta_1L_0}{C_L\delta}}, \frac{C_1\Delta_1L_1}{C_L\delta}\right\},
    \end{aligned}
\end{equation}
Given any $\epsilon>0$ and $\delta\in(0,1)$, choose
\begin{equation*}
    \begin{aligned}
        \eta \leq c_1 \cdot \min\left\{\frac{r\lambda}{G}, \frac{\lambda}{L}, \frac{\sigma_{g,1}^2G^2\delta}{\lambda\Delta_1\mu^2}, \frac{\lambda^2\sqrt{\delta}\epsilon}{\sigma_{\phi}GL}\right\},
        \quad
        0 \leq \betasq \leq 1,
        \quad
        \beta = \frac{C_2\mu^2\eta^2}{\sigma_{g,1}^2},
    \end{aligned}
\end{equation*}
\begin{equation*}
    \begin{aligned}
        \gamma = \frac{c_2\beta}{\mu\max\{1,\ln(C_{\eta})\}},
        \quad
        \nu = \sqrt{\beta},
        \quad
        I = \frac{1}{\sqrt{\beta}},
        \quad
        T = \frac{64G\Delta_1}{\eta\delta\epsilon^2},
        \quad
        S_1\geq \frac{1}{2\beta^2T},
    \end{aligned}
\end{equation*}
\begin{equation*}
    \begin{aligned}
        T_0 \geq \ln\left(\frac{\mu\gamma\eta^2}{6\|y_0-y_0^*\|^2}\right) \Big/ \ln\left(1-\frac{\sqrt{\mu\gamma}}{4}\right),
        \quad
        N \geq \ln\left(\frac{\mu\gamma\eta^2}{6(\eta + \eta l_{g,1}IC_m/\lambda\mu)^2}\right) \Big/ \ln\left(1-\frac{\sqrt{\mu\gamma}}{4}\right),
    \end{aligned}
\end{equation*}
\begin{equation*}
    \begin{aligned}
        Q \geq \frac{\ln\left(\frac{2\mu^2G\Delta_1}{\eta l_{g,1}^2l_{f,0}^2}\right)}{2\ln\left[\left(\frac{32GT}{\lambda} + \frac{32\cdot72GTl_{g,1}^2L^2}{\lambda^3\mu^2}\left(\frac{\eta^2}{\nu^2} + \eta^2I^2\right)\right) + \frac{16G}{\lambda\beta}\left(\frac{\lambda\beta}{32G} + \frac{24\eta^2L^2T}{\lambda^2}\left(1+\frac{l_{g,1}}{\mu}\right)^2\right)\right]},
    \end{aligned}
\end{equation*}
where $C_{\eta}$ is defined as
\begin{equation*}
    C_{\eta} = \frac{512e\Delta_1\sigma_{\phi}LG^2}{c_1\lambda^2\delta^{3/2}\epsilon^3}.
\end{equation*}
% where the definitions of problem-dependent constants are listed in \cref{app:notations}. 
Run \cref{alg:vradambo} for $T$ iterations. Then with probability at least $1-\delta$ over the randomness in $\gF_{T+1}$, we have $\|\gdphi(x_t)\|\leq G$ for all $t\in[T]$, and $\frac{1}{T}\sum_{t=1}^{T}\|\gdphi(x_t)\|\leq \epsilon^2$.
\end{theorem}

\begin{proof}[Proof of \cref{thm:vr-main-appendix}]
By \cref{lm:vr-three-bounds}, we have
\begin{equation*}
    \begin{aligned}
        \E\left[\sum_{t=1}^{\tau-1}\|\gdphi(x_t)\|^2\right] \leq \gI,
        \quad
        \E[\Phi(x_{\nu}) - \Phi^*] \leq \frac{\eta\gI}{8G}, 
        \quad
        \E[\|\epsilon_{\tau}\|^2] \leq \frac{\lambda\beta\gI}{16G}.
    \end{aligned}
\end{equation*}
First, note that if $\tau=\tau_1\leq T$, we know $\Phi(x_{\tau})-\Phi^* > \psi$ by the definition of $\tau$. Then we have
\begin{equation*}
    \begin{aligned}
        \pr(\tau=\tau_1\leq T) \leq \pr(\Phi(x_{\tau})-\Phi^* > \psi) \leq \frac{\E[\Phi(x_{\tau})-\Phi^*]}{\psi} \leq \frac{\eta\gI}{8G\psi} = \frac{\eta L\gI}{4C_LG^3},
    \end{aligned}
\end{equation*}
where the second inequality uses Markov's inequality. \eqref{eq:psi-def}

Similarly, if $\tau_2=\tau\leq T$, we know $\|\epsilon_t\|> G$ by the definition of $\tau$. Then we also have
\begin{equation*}
    \begin{aligned}
        \pr(\tau=\tau_2\leq T) \leq \pr(\|\epsilon_{\tau}\|>G) = \pr(\|\epsilon_{\tau}\|^2 > G^2) \leq \frac{\E[\|\epsilon_{\tau}\|^2]}{G^2} \leq \frac{\lambda\beta\gI}{16G^3}.
    \end{aligned}
\end{equation*}
% In other words, there exists events $\gE_1$ and $\gE_2$ such that 
Under event $\gE_y$, we further have
\begin{equation} \label{eq:gI-bound}
    \begin{aligned}
        \gI \leq \frac{16G\Delta_1}{\eta},
    \end{aligned}
\end{equation}
which implies that
\begin{equation*}
    \begin{aligned}
        \frac{\eta L\gI}{4C_LG^3} \leq \frac{4\Delta_1L}{C_LG^2} = \frac{4\Delta_1L_0}{C_LG^2} + \frac{4\Delta_1L_1}{C_LG} \leq \frac{8\delta}{C_1} \leq \frac{\delta}{16},
    \end{aligned}
\end{equation*}
where the first equality use the definition of $L$, the second inequality is due to the choice of $G$, and in the last inequality we choose large enough $C_1$; \eqref{eq:gI-bound} also implies that
\begin{equation*}
    \begin{aligned}
        \frac{\lambda\beta\gI}{16G^3} \leq \frac{\lambda\beta\Delta_1}{\eta G^2} = \frac{C_2\lambda\mu^2\Delta_1\eta}{\sigma_{g,1}^2G^2} \leq c_1C_2\delta \leq \frac{\delta}{16},
    \end{aligned}
\end{equation*}
where the first equality uses the choice of $\beta$, the second inequality is due to the choice of $\eta$, and in the last inequality we choose small enough $c_1$. Thus, we obtain for $i=1,2$ that
\begin{equation*}
    \begin{aligned}
        \pr(\tau=\tau_i\leq T)
        &= \pr(\tau=\tau_i\leq T \mid \gE_y)\pr(\gE_y) + \pr(\tau=\tau_i\leq T \mid \gE_y^{c})\pr(\gE_y^{c}) \\
        &\leq \frac{\delta}{16}\left(1-\frac{\delta}{8}\right) + \frac{\delta}{8}
        \leq \frac{3\delta}{16}.
    \end{aligned}
\end{equation*}
Therefore, we have
\begin{equation*}
    \begin{aligned}
        \pr(\tau\leq T)
        \leq \pr(\tau=\tau_1\leq T) + \pr(\tau=\tau_2\leq T)
        \leq \frac{3\delta}{8}.
    \end{aligned}
\end{equation*}
Also, note that by \cref{lm:vr-three-bounds} we have
\begin{equation*}
    \begin{aligned}
        \gI 
        &\geq \E\left[\sum_{t=1}^{\tau-1}\|\gdphi(x_t)\|^2\right] \\
        &\geq \pr(\{\tau = T+1\}\cap\gE_y)\E\left[\sum_{t=1}^{T}\|\gdphi(x_t)\|^2 \mid \{\tau = T+1\}\cap\gE_y\right] \\
        &\geq \frac{1}{2}\E\left[\sum_{t=1}^{T}\|\gdphi(x_t)\|^2 \mid \{\tau = T+1\}\cap\gE_y\right],
    \end{aligned}
\end{equation*}
where the last inequality uses 
\begin{equation*}
    \begin{aligned}
        \pr(\{\tau = T+1\}\cap\gE_y)
        &= 1 - \pr(\{\tau\leq T\}\cup\gE_y^{c}) \\
        &\geq 1 - \pr(\tau\leq T) - \pr(\gE_y^{c})
        \geq 1 - \frac{3\delta}{8} - \frac{\delta}{8}
        = 1 - \frac{\delta}{2}
        \geq \frac{1}{2}.
    \end{aligned}
\end{equation*}
Then we obtain 
\begin{equation} \label{eq:apply-markov}
    \begin{aligned}
        \E\left[\frac{1}{T}\sum_{t=1}^{T}\|\gdphi(x_t)\|^2 \mid \{\tau = T+1\}\cap\gE_y\right]
        \leq 2\gI \leq \frac{32G\Delta_1}{\eta T} \leq \frac{\delta\epsilon^2}{2},
    \end{aligned}
\end{equation}
where the second inequality uses \eqref{eq:gI-bound}, and the last inequality is due to the choice of $T$. Now we define $\gE^{c}$ to be the event that \cref{alg:vradambo} does not converge to $\epsilon$-stationary points:
\begin{equation*}
    \begin{aligned}
        \gE^{c} \coloneqq \left\{\frac{1}{T}\sum_{t=1}^{T}\|\gdphi(x_t)\|^2 > \epsilon^2\right\}.
    \end{aligned}
\end{equation*}
By \eqref{eq:apply-markov} and Markov's inequality, we have
\begin{equation*}
    \begin{aligned}
        \pr(\gE^{c} \mid \{\tau = T+1\}\cap\gE_y)
        \leq \frac{\delta\epsilon^2}{2\epsilon^2} = \frac{\delta}{2}.
    \end{aligned}
\end{equation*}
Then we have
\begin{equation*}
    \begin{aligned}
        \pr(\gE^{c}\cup\{\tau\leq T\}\cup\gE_y^{c}) 
        &\leq \pr(\{\tau\leq T\}\cup\gE_y^{c}) + \pr(\gE^{c} \mid \{\tau = T+1\}\cap\gE_y) \\
        &\leq \pr(\{\tau\leq T\}) + \pr(\gE_y^{c}) + \pr(\gE^{c} \mid \{\tau = T+1\}\cap\gE_y) \\
        &\leq \frac{3\delta}{8} + \frac{\delta}{8} + \frac{\delta}{2}
        = \delta,
    \end{aligned}
\end{equation*}
which yields 
\begin{equation*}
    \begin{aligned}
        \pr(\gE\cap\{\tau=T+1\}\cap\gE_y) = 1 - \pr(\gE^{c}\cup\{\tau\leq T\}\cup\gE_y^{c}) \geq 1-\delta.
    \end{aligned}
\end{equation*}
Therefore, we conclude that with probability at least $1-\delta$, we have $\tau=T+1$ and $\|\gdphi(x_t)\|\leq G$ for all $t\in[T]$, and $\frac{1}{T}\sum_{t=1}^{T}\|\gdphi(x_t)\|^2\leq \epsilon^2$.
\end{proof}

%%%%%%%%%%%%%%%%%%%%%%%%%%%%%%%%%%%%%%%%%%%%%%%%%%%%%%%%%%%%%%%%%%%%%%%%%%%%%%%%%%%%%%%%%%%%%%%
\subsection{Parameter Choices for VR-AdamBO (\cref{thm:vr-main-appendix})}
\label{sec:vr-para-verify}

We first list all the relevant parameter choices below for convenience:
\begin{equation*}
    \begin{aligned}
        G \geq \max\left\{4\lambda, 2\sigma_{\phi}, 4C_{\phi,0}, \frac{C_{\phi,1}}{L_1}, \sqrt{\frac{C_1\Delta_1L_0}{C_L\delta}}, \frac{C_1\Delta_1L_1}{C_L\delta}\right\},
        \quad
        C_{\eta} = \frac{512C_3e\Delta_1\sigma_{\phi}LG^2}{c_1\lambda^2\delta^{3/2}\epsilon^3},
    \end{aligned}
\end{equation*}
\begin{equation*}
    \begin{aligned}
        \eta \leq c_1 \cdot \min\left\{\frac{r\lambda}{G}, \frac{\lambda}{L}, \frac{\lambda^2\delta}{\Delta_1L^2}, \frac{\lambda^2\sqrt{\delta}\epsilon}{\sigma_{\phi}GL}\right\},
        \quad
        0 \leq \betasq \leq 1,
        \quad
        \beta = \frac{C_2\mu^2\eta^2}{\sigma_{g,1}^2},
        % \beta = \frac{C_2^2\eta^2}{\max\{1,\ln(C_{\eta})\}}, 
    \end{aligned}
\end{equation*}
\begin{equation*}
    \begin{aligned}
        % 0 \leq \betasq \leq 1,
        % \quad
        % \beta = C_2^2\eta^2, 
        % \quad
        \gamma = \frac{c_2\beta}{\mu\max\{1,\ln(C_{\eta})\}},
        \quad
        \nu = \sqrt{\beta},
        \quad
        I = \frac{1}{\sqrt{\beta}},
        \quad
        T = \frac{C_3G\Delta_1}{\eta\delta\epsilon^2},
        \quad
        S_1\geq \frac{1}{2\beta^2T},
    \end{aligned}
\end{equation*}
\begin{equation*}
    \begin{aligned}
        T_0 \geq \ln\left(\frac{\mu\gamma\eta^2}{6\|y_0-y_0^*\|^2}\right) \Big/ \ln\left(1-\frac{\sqrt{\mu\gamma}}{4}\right),
        \quad
        N \geq \ln\left(\frac{\mu\gamma\eta^2}{6(\eta + \eta l_{g,1}IC_m/\lambda\mu)^2}\right) \Big/ \ln\left(1-\frac{\sqrt{\mu\gamma}}{4}\right),
    \end{aligned}
\end{equation*}

\paragraph{Verification for \cref{lm:sum-hy-and-y}.}
By choices of $\eta, \beta, \nu$ and $I$, we have
\begin{equation*}
    \begin{aligned}
        \frac{36l_{g,1}^2L^2}{\lambda^2\mu^2}\left(\frac{\eta^2}{\nu^2} + \eta^2I^2\right) 
        &= \frac{72\eta^2l_{g,1}^2L^2}{\lambda^2\mu^2\beta} 
        = \frac{72\sigma_{g,1}^2l_{g,1}^2L^2}{C_2\lambda^2\mu^4} 
        \leq \frac{1}{2},
    \end{aligned}
\end{equation*}
where in the last inequality we choose large enough $C_2$.

\paragraph{Verification for \cref{lm:vr-three-bounds}.}
By choices of $\eta, \beta, \nu$ and $I$, we have
\begin{equation*}
    \begin{aligned}
        \frac{32\cdot72Gl_{g,1}^2L^2}{\lambda^3\mu^2}\left(\frac{\eta^2}{\nu^2} + \eta^2I^2\right)
        &= \frac{32\cdot72\eta^2Gl_{g,1}^2L^2}{\lambda^3\mu^2\beta} 
        = \frac{32\cdot72G\sigma_{g,1}^2l_{g,1}^2L^2}{C_2\lambda^3\mu^4} 
        \leq \min\left\{\frac{1}{4}, \frac{4G}{\lambda}\right\},
    \end{aligned}
\end{equation*}
where in the last inequality we choose large enough $C_2$.

\paragraph{Verification for \cref{lm:first-window,lm:general-window}.}
Similar to \cref{app:proof_biadam}, we focus on the dominant terms for each parameter choice when $\epsilon$ is sufficiently small. For the remaining cases, the result can be easily obtained by following the same procedure. Specifically, we consider the case where $\eta$ is chose as 
\begin{equation*}
    \eta = \frac{c_1\lambda^2\sqrt{\delta}\epsilon}{\sigma_{\phi}GL}.
\end{equation*}
Under event $\gE_y$, by \cref{lm:first-window} we have
\begin{equation*}
    \begin{aligned}
        \|y_1-y_0^*\|^2
        &\leq \frac{3}{\mu\gamma}\left(1-\frac{\sqrt{\mu\gamma}}{4}\right)^{T_0}\|y_0-y_0^*\|^2 + \frac{4\gamma\sigma_{g,1}^2}{\mu}\ln\frac{8eT}{\delta} 
        \leq \frac{\eta^2}{2} + \frac{4c_2\beta\sigma_{g,1}^2}{\mu^2\max\{1,\ln(C_{\eta})\}}\ln(C_{\eta}) \\
        &= \frac{\eta^2}{2} + \frac{4c_2C_2\eta^2}{\ln(C_{\eta})}\ln(C_{\eta}) 
        \leq \frac{\eta^2}{2} + \frac{\eta^2}{2}
        = \eta^2,
    \end{aligned}
\end{equation*}
where the second inequality uses the choices of $T_0$ and $\gamma$, the third inequality is due to the choice of $\beta$, and in the last inequality we choose small enough $c_2$.

Under event $\gE_y$, by \cref{lm:general-window}, for $k\geq 1$ we have
\begin{equation*}
    \begin{aligned}
        \|y_{kI+1}-y_{kI}^*\|^2
        &\leq \frac{3}{\mu\gamma}\left(1-\frac{\sqrt{\mu\gamma}}{4}\right)^{N}\|y_{kI}-y_{kI}^*\|^2 + \frac{4\gamma\sigma_{g,1}^2}{\mu}\ln\frac{8eT}{\delta} \\
        &\leq \frac{3}{\mu\gamma}\left(1-\frac{\sqrt{\mu\gamma}}{4}\right)^{N}\left(\eta + \frac{\eta l_{g,1}I}{\lambda\mu}C_m\right)^2 + \frac{\eta^2}{2} 
        \leq \frac{\eta^2}{2} + \frac{\eta^2}{2}
        = \eta^2,
    \end{aligned}
\end{equation*}
where the third inequality uses the choice of $N$.

\paragraph{Verification for $\|\hy_t-y_t^*\|\leq \hrho\leq \min\{r,1/4L_1\}$.}
First, by choices of $\eta,\nu$ and $I$, we have
\begin{equation*}
    \begin{aligned}
        \frac{\eta l_{g,1}L}{\lambda\mu}\left(\frac{1-\nu}{\nu} + I\right)
        &\leq \frac{l_{g,1}L}{\lambda\mu}\left(\frac{\eta}{\nu} + \eta I\right) 
        = \frac{2\eta l_{g,1}L}{\lambda\mu\sqrt{\beta}} \\
        &\leq \frac{2\sigma_{g,1}l_{g,1}L}{\sqrt{C_2}\lambda\mu^2} 
        \leq \frac{1}{2},
    \end{aligned}
\end{equation*}
where in the last inequality we choose large enough $C_2$. Under event $\gE_y$, by \cref{lm:general-window} we have
\begin{equation*}
    \begin{aligned}
        \|\hy_t-y_t^*\|
        &\leq \hrho \\
        &= \left(\|\hy_1-y_0^*\| + \eta + \frac{\eta l_{g,1}}{\lambda\mu}\left(\frac{1-\nu}{\nu} + I\right)\left(2G + \frac{l_{g,1}l_{f,0}}{\mu}\right)\right) \Big/ \left(1-\frac{\eta l_{g,1}L}{\lambda\mu}\left(\frac{1-\nu}{\nu} + I\right)\right) \\
        &\leq 2\left(2\eta + \frac{\eta l_{g,1}}{\lambda\mu}\left(\frac{1-\nu}{\nu} + I\right)\left(2G + \frac{l_{g,1}l_{f,0}}{\mu}\right)\right) \\
        &\leq 2\left(\frac{2c_1r\lambda}{G} + \frac{2\sigma_{g,1}l_{g,1}L}{\sqrt{C_2}\lambda\mu^2}\left(2G + \frac{l_{g,1}l_{f,0}}{\mu}\right)\right) 
        \leq \min\left\{r, \frac{1}{4L_1}\right\},
    \end{aligned}
\end{equation*}
where the second inequality uses $\|\hy_1-y_0^*\|\leq \eta$, the third inequality is due to the choices of $\eta,\nu$ and $I$, and in the last inequality we choose small enough $c_1$ and large enough $C_2$. Therefore, we also have
\begin{equation*}
    \begin{aligned}
        C_m 
        = 2G + \frac{l_{g,1}l_{f,0}}{\mu} + L\hrho 
        \leq 2G + \frac{l_{g,1}l_{f,0}}{\mu} + Lr.
    \end{aligned}
\end{equation*}

\paragraph{Verification for \cref{lm:vr-momentum-error-sum}.}
By choices of $\eta, \beta, \nu$ and $I$, we have
\begin{equation*}
    \begin{aligned}
        48L^2\left(\nu^2 + \frac{\lambda\beta}{400G}\right) \cdot \frac{72l_{g,1}^2L^2}{\lambda^2\mu^2}\left(\frac{\eta^2}{\nu^2} + \eta^2I^2\right)
        &= \frac{48\cdot144\sigma_{g,1}^2l_{g,1}^2L^4}{C_2\lambda^2\mu^4}\left(1 + \frac{\lambda}{400G}\right)\beta
        \leq \frac{\lambda\beta}{64G},
    \end{aligned}
\end{equation*}
where in the last inequality we choose large enough $C_2$. We also have
\begin{equation*}
    \begin{aligned}
        24\nu^2L^2 \cdot \frac{8\eta^2l_{g,1}^2I^2}{\lambda^2\mu^2}\left(1 + \frac{72l_{g,1}^2L^2}{\lambda^2\mu^2}\left(\frac{\eta^2}{\nu^2} + \eta^2I^2\right)\right) 
        \leq \frac{192\sigma_{g,1}^2l_{g,1}^2L^2}{C_2\lambda^2\mu^4}\left(1 + \frac{72\sigma_{g,1}^2l_{g,1}^2L^2}{C_2\lambda^2\mu^4}\right)\beta 
        \leq \frac{\lambda\beta}{64G},
    \end{aligned}
\end{equation*}
where in the last inequality we choose large enough $C_2$. In addition, under event $\gE_y$, we have
\begin{equation*}
    \begin{aligned}
        &\left(\left(1+\frac{\nu l_{g,1}}{\mu}\right)\frac{\eta}{\lambda} + \frac{\nu\eta l_{g,1}I}{\lambda\mu}\right)\max_{t\leq T}\|m_t\| + \nu(\varrho_{\max} + \hrho_{\max}) \\
        &\leq \left(\frac{1}{\lambda} + \frac{2l_{g,1}}{\lambda\mu}\right)C_m\eta + \sqrt{\beta}(\eta + \varrho) \\
        &\leq \left(\frac{1}{\lambda} + \frac{2l_{g,1}}{\lambda\mu}\right)\left(2G + \frac{l_{g,1}l_{f,0}}{\mu} + Lr\right)\eta + \frac{\sqrt{C_2}\mu\eta}{\sigma_{g,1}}\left(1+\frac{c_1\lambda}{G}\right)r \\
        &\leq \left(\frac{1}{\lambda} + \frac{2l_{g,1}}{\lambda\mu}\right)\left(2G + \frac{l_{g,1}l_{f,0}}{\mu} + Lr\right)\frac{c_1\lambda}{L} + \frac{c_1\sqrt{C_2}\mu\lambda}{\sigma_{g,1}L}\left(1+\frac{c_1\lambda}{G}\right)r 
        \leq r,
    \end{aligned}
\end{equation*}
where the first inequality uses \cref{lm:general-window,lm:first-window} such that $\max_{t\leq T}\|m_t\|\leq C_m$, $\varrho_{\max}\leq \eta$ and $\hrho_{\max}\leq \hrho$; the second inequality is due to the choices of $\eta$ and $\beta$, and $\hrho\leq r$; and in the last inequality we use the choice of $\eta$ again and choose small enough $c_1$.

\paragraph{Verification for \cref{thm:vr-main-appendix}.}
Under event $\gE_y$, by \cref{lm:vr-three-bounds} we have
\begin{equation*}
    \begin{aligned}
        \gI
        &= \frac{8G\Delta_1}{\eta} + \frac{128G\sigma_{\phi}^2\beta T}{\lambda} + \left(\frac{32GL^2}{\lambda} + \frac{16\cdot48GL^2}{\lambda\beta}\left(\nu^2 + \frac{\lambda\beta}{400G}\right)\right)\left(\frac{6}{\nu}\|\hy_1-y_0^*\|^2 + 12\varrho_{\max}^2T\right) \\
        &\quad+ \frac{16\cdot24\nu^2GL^2}{\lambda\beta}\left(\frac{48\eta^2l_{g,1}^2I^2L^2}{\nu\lambda^2\mu^2}\|\hy_1-y_0^*\|^2 + \left(2 + \frac{96\eta^2l_{g,1}^2I^2L^2}{\lambda^2\mu^2}\right)\varrho_{\max}^2T\right) \\
        &\quad+ \left[\left(\frac{32GT}{\lambda} + \frac{32\cdot72GTl_{g,1}^2L^2}{\lambda^3\mu^2}\left(\frac{\eta^2}{\nu^2} + \eta^2I^2\right)\right) \right.\\
        &\left.\quad+ \frac{16G}{\lambda\beta}\left(\frac{\lambda\beta}{32G} + \frac{24\eta^2L^2T}{\lambda^2}\left(1+\frac{l_{g,1}}{\mu}\right)^2\right)\right]\frac{l_{g,1}^2l_{f,0}^2}{\mu^2}\left(1-\frac{\mu}{l_{g,1}}\right)^{2Q}
        \leq \frac{16G\Delta_1}{\eta} \\
        &\leq \frac{8G\Delta_1}{\eta} + \frac{128G\sigma_{\phi}^2\beta T}{\lambda} + \left(\frac{32GL^2}{\lambda} + \frac{16\cdot48GL^2}{\lambda\beta}\left(\nu^2 + \frac{\lambda\beta}{400G}\right)\right)\left(\frac{6\eta^2}{\nu} + 12\eta^2T\right) \\
        &\quad+ \frac{16\cdot24\nu^2GL^2}{\lambda\beta}\left(\frac{48\eta^4l_{g,1}^2I^2L^2}{\nu\lambda^2\mu^2} + \left(2 + \frac{96\eta^2l_{g,1}^2I^2L^2}{\lambda^2\mu^2}\right)\eta^2T\right) + \frac{2G\Delta_1}{\eta} \\
        &\leq \frac{16G\Delta_1}{\eta},
    \end{aligned}
\end{equation*}
where the first inequality uses the choice of $Q$ and the fact that under event $\gE_y$, $\varrho_{\max}\leq \eta$ by \cref{lm:first-window}, and in the last inequality we plug in the choices of $\beta, \eta, \nu, I, T$ and choose small enough $c_1,c_2$ and large enough $C_1,C_2$ to obtain the final bound for $\gI$.
